# Supplementary material for: MVFNet: Multipurpose Video Forensics Network using Multiple Forms of Forensic Evidence
Source: arXiv:2503.20991 source file (2025-03-26)
Supplement: Supplementary file 1 [file Supp_FFE_Pretraining.tex]

\section{Forensic Residual Feature Extractor Pretraining}

We introduce a novel pretraining procedure for the Forensic Residual Feature Extractor (FRFE) by building upon the established method in multimedia forensics for obtaining general forensic features through training on the Camera Model ID task~\cite{MISLnet, EXIFnet, Noiseprint, FSG, FSM}. Our innovation lies in the means of producing forensic embeddings, and a new, accompanying objective function. The input frame initially passes through the FRFE's trunk, which includes its constrained convolutional layer and its series of FIR blocks (see Fig.~\ref{fig:ffe_arch}). In prior works~\cite{VideoFACT, MISLnet, EXIFnet, Noiseprint, FSG, FSM}, this set of features is often condensed into a single embedding vector representing the entire frame for classification. However, in our work, we aggregated forensic features into embeddings for each analysis windows at multiple scales using a multi-resolution pooling module, as described in Sec.~\ref{subsec:multi_res_joint_embedding}. The resulting embeddings at each scale are then parallelly put through their own classification heads to produce 2D maps, in which each element specifies the input frame's camera model class. The learning objective is to ensure that all elements in this map correspond to the same true camera model class, promoting consistency across all spatial embeddings at different scales.
\begin{comment}
The loss function for each scale is defined as:
\begin{equation}
	\mathcal{L}_{\text{ffe}}^{(k)} = -\frac{1}{2^k \times 2^k} \sum_{i,j} \sum_{c}
	\log(\frac{\exp(M^{k,c}_{i,j})}{\sum_{c} \exp(M^{k,c}_{i,j})} \cdot \mathbbm{1}_{c=C})
\end{equation}
where $M^{k,c}_{i,j}$ is the classification map at scale $k$ and CM $c$, and $\mathbbm{1}_{c=C}$ is the indicator function that is 1 when $c$ is the correct CM $C$ and 0 otherwise.
\end{comment}
The overall pretraining loss combines these scale-losses into a weighted sum:
\begin{equation}
	\mathcal{L}_{\text{F}} = \sum_{k} \frac{-\lambda_k}{2^{2k}} \sum_{i,j} \sum_{c}
	\log\left(\frac{\exp(\theta^{k,c}_{i,j})\mathbbm{1}(c=c^*)}{\sum_{c} \exp(\theta^{k,c}_{i,j})} %\mathbbm{1}_{c=c^*}
	\right)
\end{equation}
%\begin{equation}
%	\mathcal{L}_{\text{ffe}} = \sum_{k=1}^{K} w_{k} \mathcal{L}_{\text{ffe}}^{(k)}
%\end{equation}
with $\theta^{k,c}_{i,j}$ being the classification map at scale $k$, camera model $c$, and $\mathbbm{1}(c=c^*)$ being the indicator function that is 1 when $c$ is the correct camera model $c^*$ and 0 otherwise. During pretraining, we chose $k=\{3, 4, 5\}$ and $\lambda_k=\{0.01, 0.0075, 0.005\}$.
Post-training, we retain solely the trunk of the FFE and merge it into our larger network. This innovative pretraining method enhances the FFE’s capability for spatial inconsistency detection, significantly improving our ability to detect and localize spatial anomalies.
