# Supplementary material for: MVFNet: Multipurpose Video Forensics Network using Multiple Forms of Forensic Evidence
Source: arXiv:2503.20991 source file (2025-03-26)
Supplement: Supplementary file 3 [file supp_result_deepfake_dfd.tex]

\newpage
\begin{figure*}[t]
	\centering
	\includegraphics[width=1.0\linewidth]{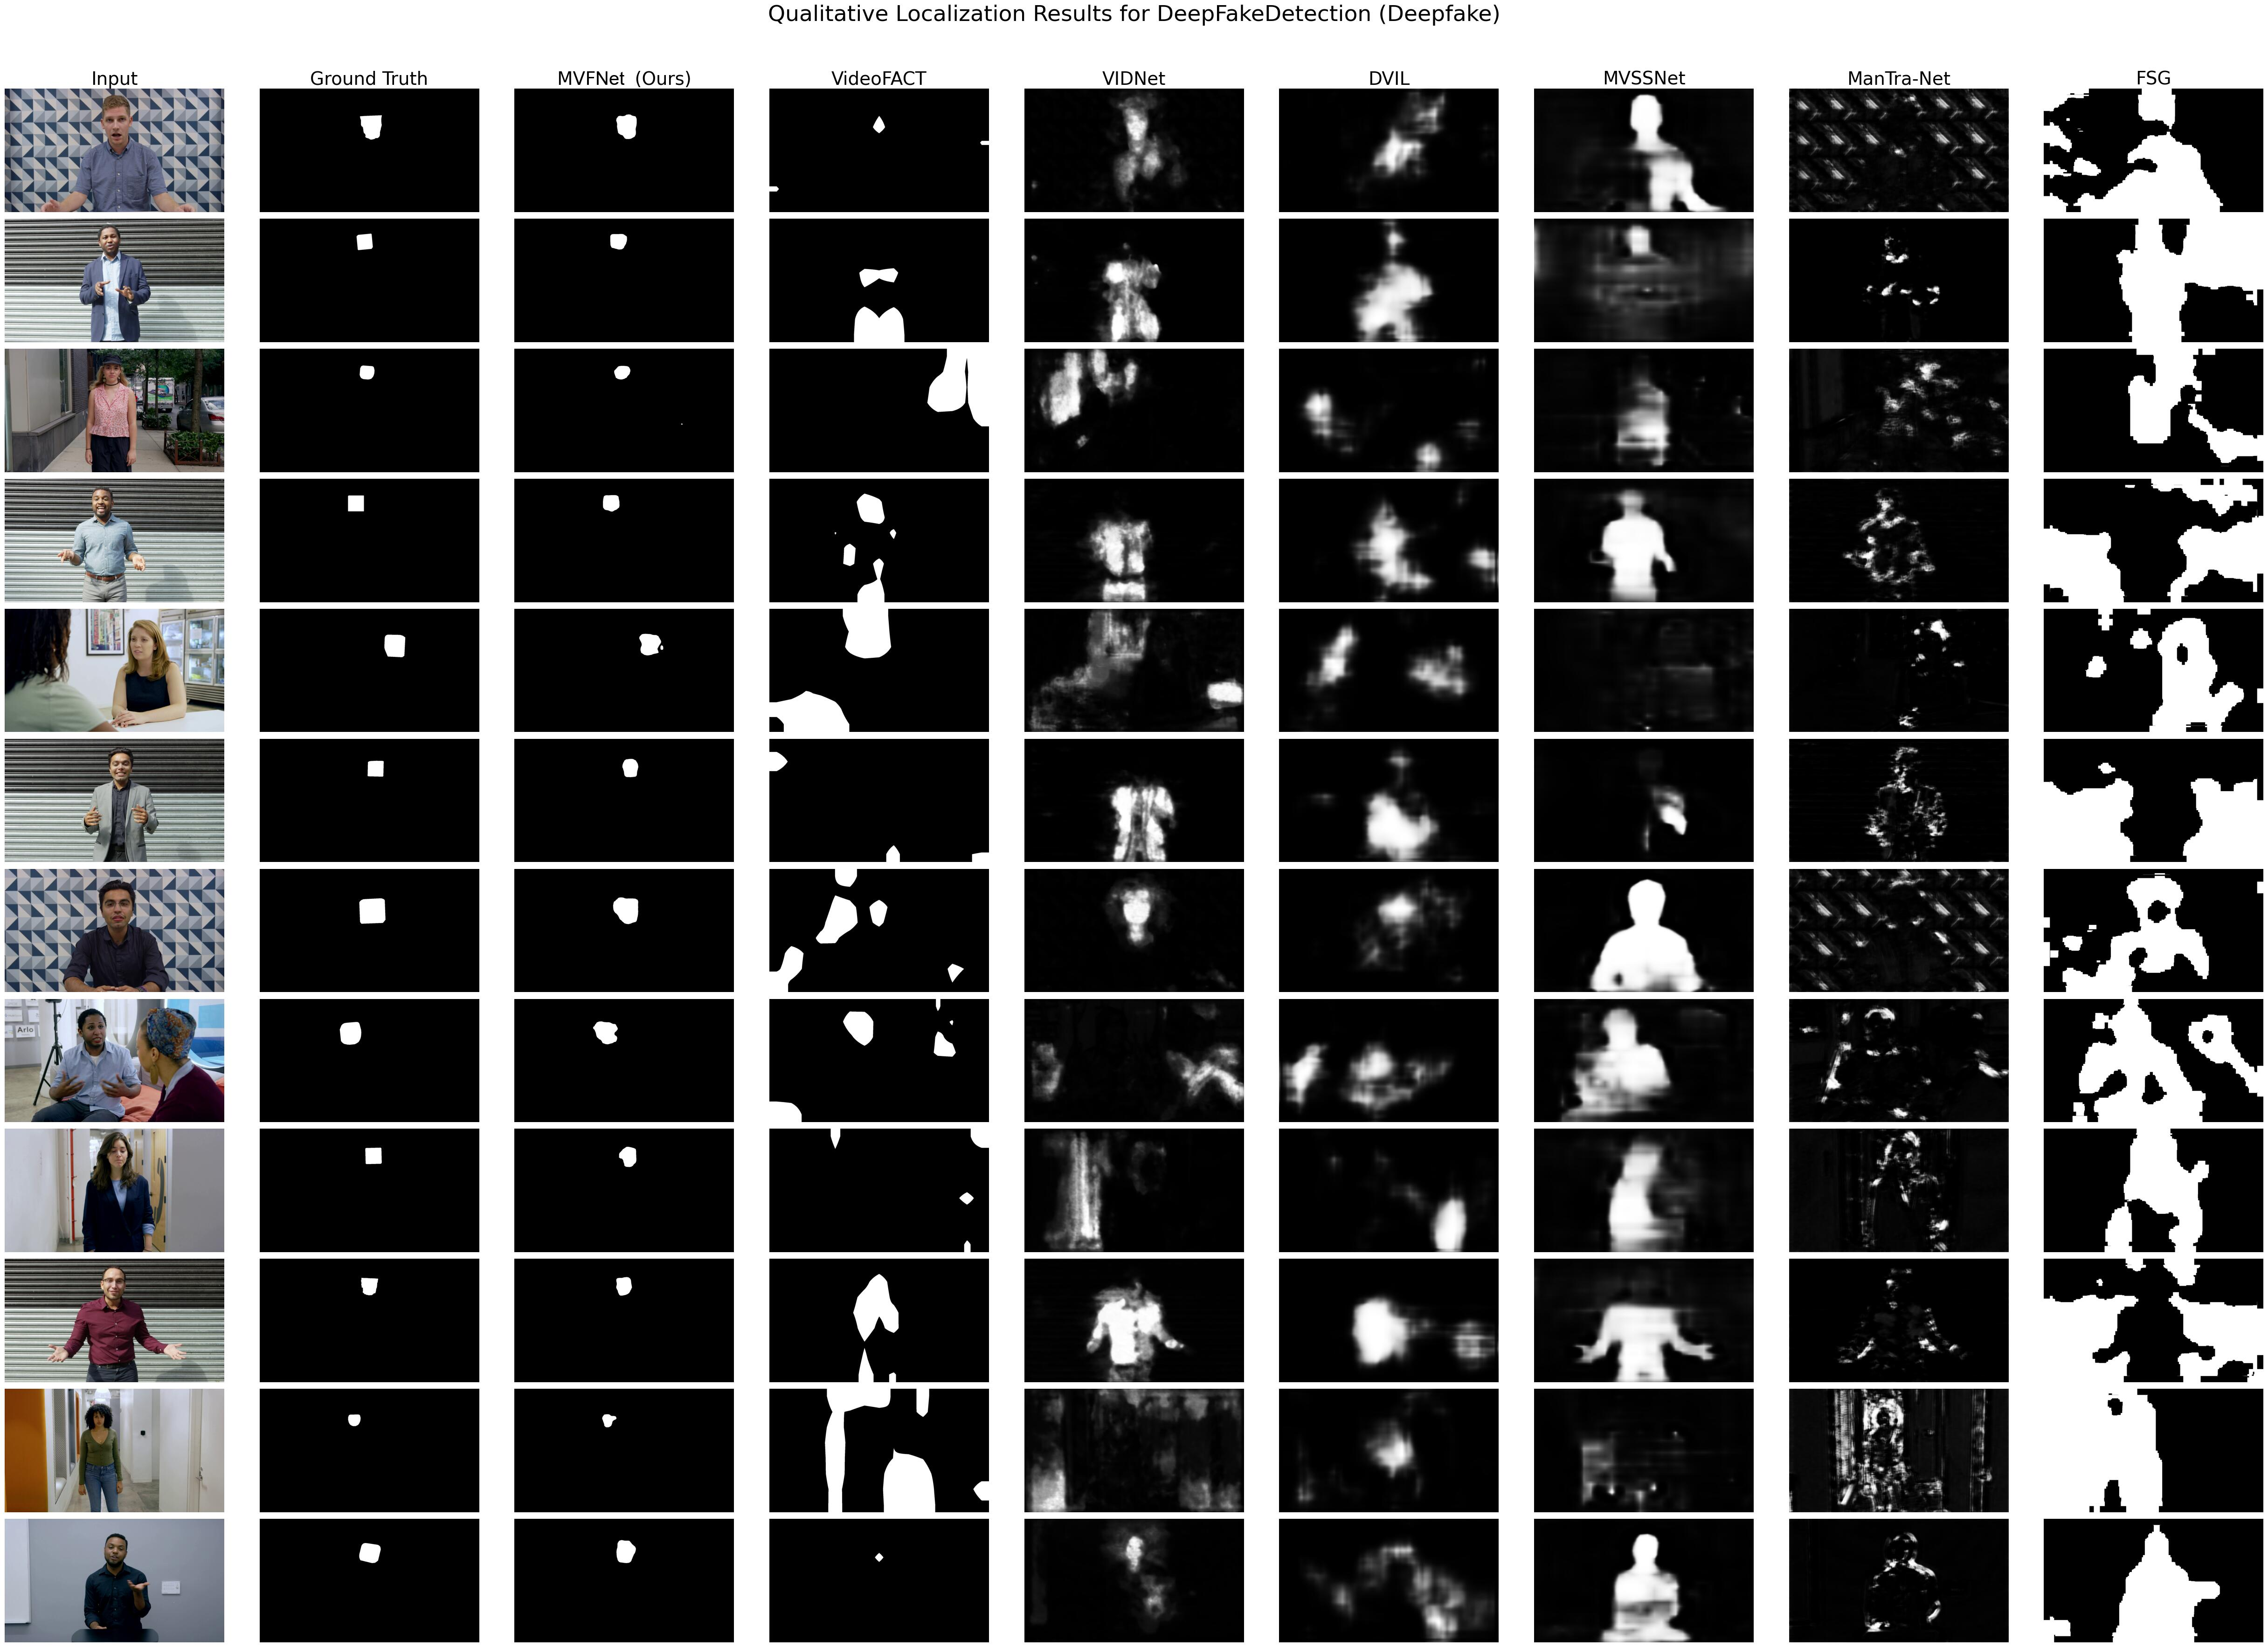}

	\vspace*{-0.5\baselineskip}

	\caption{Localization results for deepfake detection are illustrated, highlighting the comparative effectiveness of various methods. Our \ournetworkname approach consistently provides precise localizations that closely match the Ground Truth. VideoFACT shows a small degree of accuracy. VIDNet achieves correct localization sporadically, with success in very few select cases. The remaining methods—DVIL, MVSS-Net, ManTra-Net, and FSG—largely fail to localize the specific regions of manipulation, often erroneously marking either the entire body or unrelated areas within the frame.}

	\label{fig:supp_loc_res_dfd}

	\vspace*{-0.5\baselineskip}

\end{figure*}
\newpage
