# Supplementary material for: MVFNet: Multipurpose Video Forensics Network using Multiple Forms of Forensic Evidence
Source: arXiv:2503.20991 source file (2025-03-26)
Supplement: Supplementary file 4 [file supp_result_deepfake_f2f.tex]

\newpage
\begin{figure*}[t]
	\centering
	\includegraphics[width=1.0\linewidth]{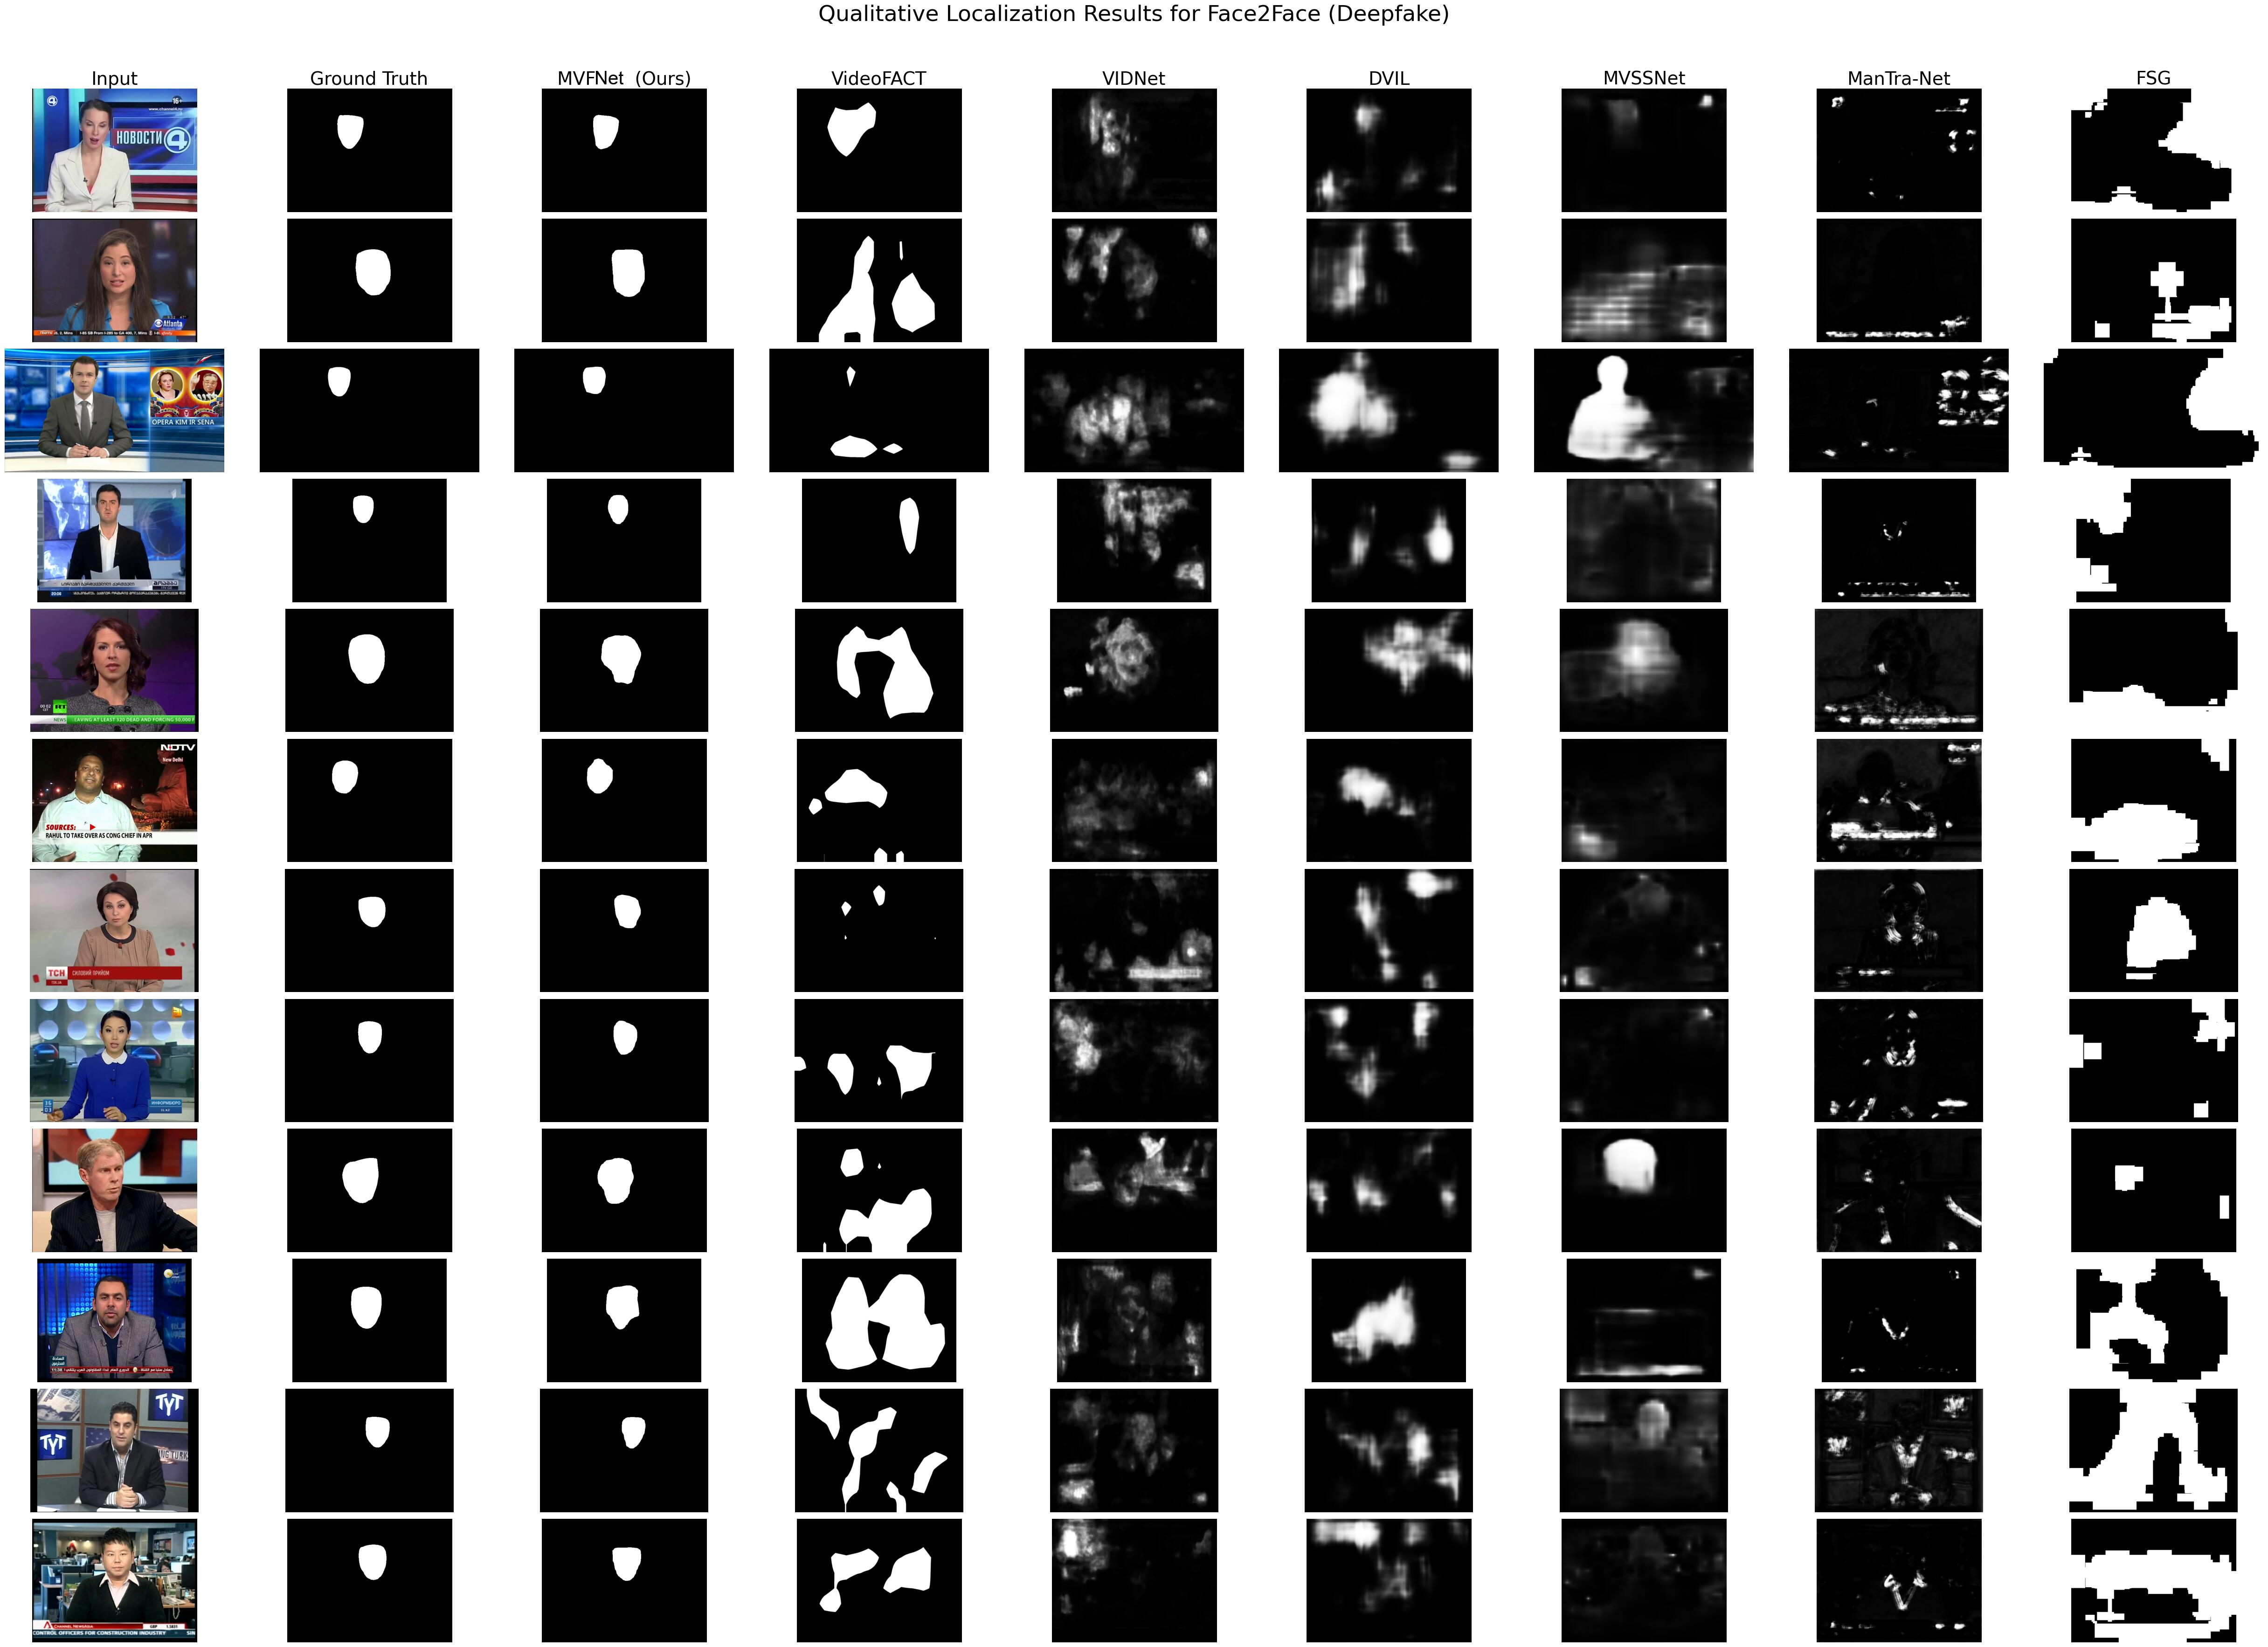}

%	\vspace*{-0.5\baselineskip}

	\caption{The figure displays localization results for Face2Face deepfake detection, highlighting the superior performance of our \ournetworkname method, which consistently provides accurate localizations that closely match the Ground Truth. VideoFACT rarely captures the manipulated regions correctly, often missing the mark. VIDNet and DVIL achieve limited success, with correct localization in a minority of cases. The rest of the methods, including MVSS-Net, ManTra-Net, and FSG, largely fail to identify the manipulated areas accurately, with localizations that either miss or misattribute the forgeries.}

	\label{fig:supp_loc_res_f2f}

%	\vspace*{-0.5\baselineskip}

\end{figure*}
\newpage
