# Supplementary material for: MVFNet: Multipurpose Video Forensics Network using Multiple Forms of Forensic Evidence
Source: arXiv:2503.20991 source file (2025-03-26)
Supplement: Supplementary file 5 [file supp_result_deepfake_fsh.tex]

\newpage
\begin{figure*}[t]
	\centering
	\includegraphics[width=1.0\linewidth]{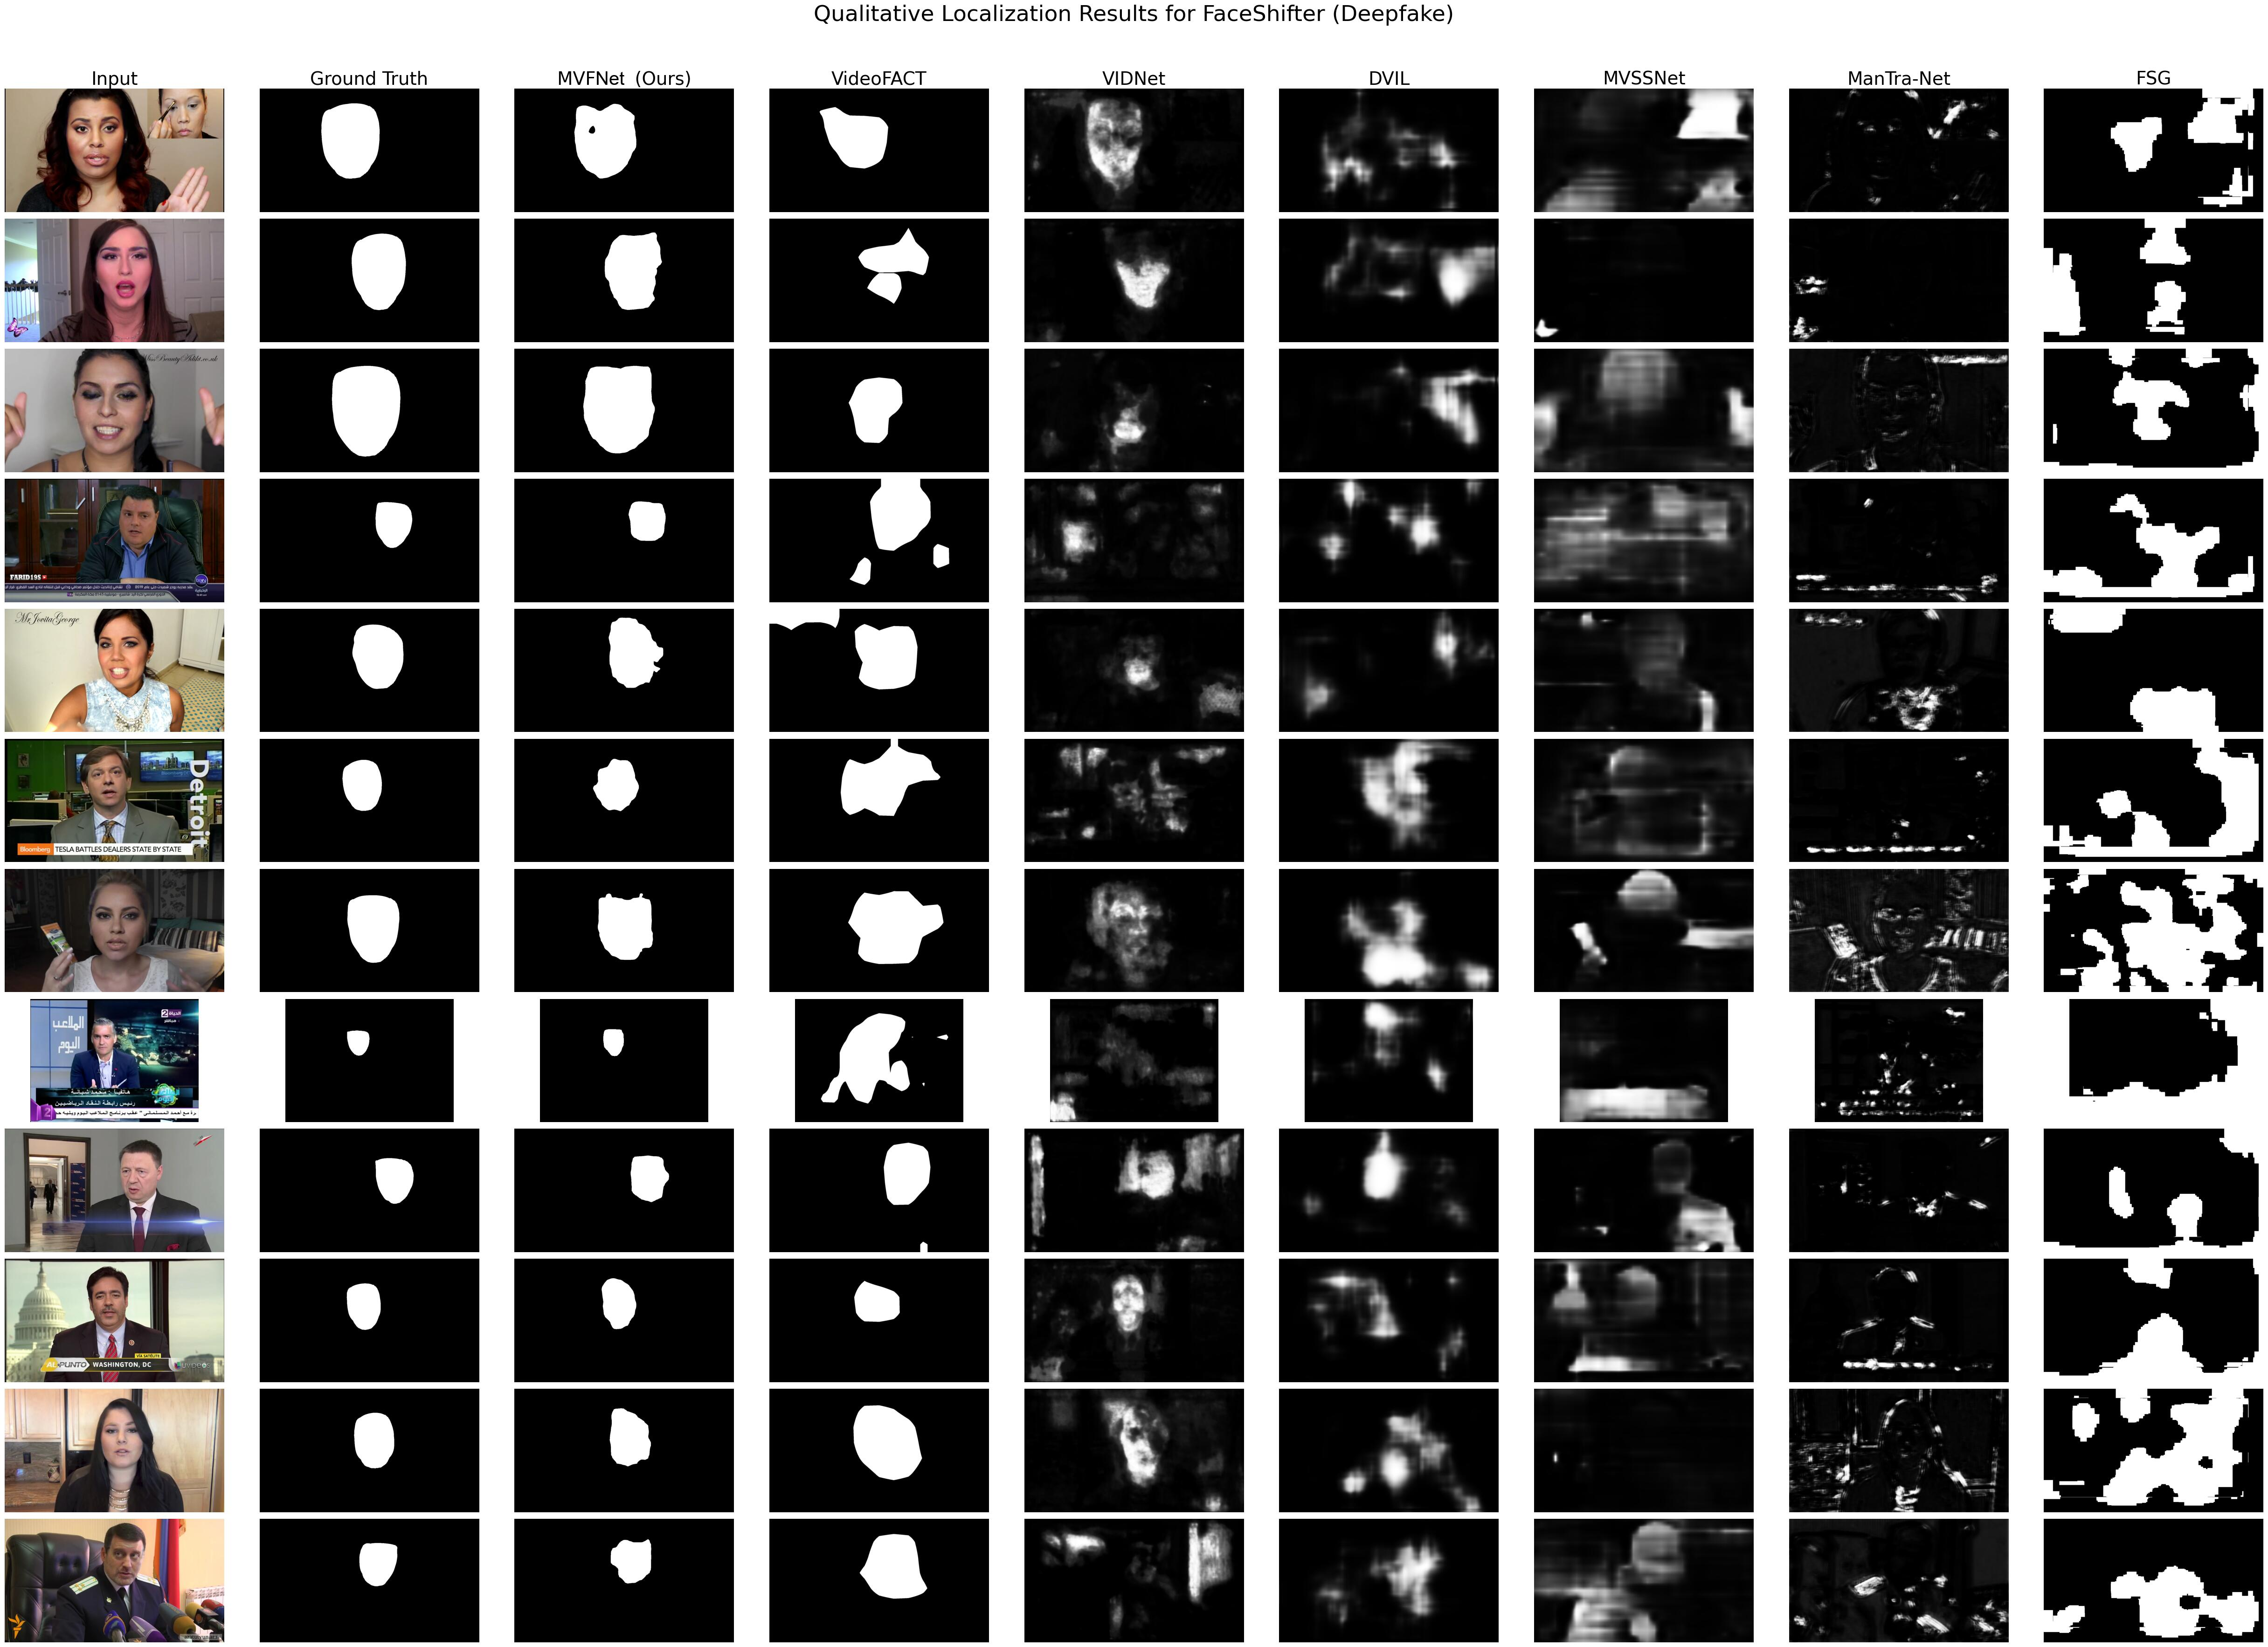}

%	\vspace*{-0.5\baselineskip}

	\caption{Comparative localization results for FaceShifter deepfake detection are depicted. Our \ournetworkname method demonstrates precise localization, closely aligning with the Ground Truth, while VideoFACT shows some capability to localize manipulated areas but with less specificity. VIDNet, although occasionally accurate, largely fails to consistently delineate the manipulated regions. DVIL, MVSS-Net, and ManTra-Net generally misidentify the extent of the manipulations, often erroneously attributing them to other areas or the entire body. FSG's localizations are overly broad and imprecise, significantly deviating from the targeted manipulations indicated by the Ground Truth.}

	\label{fig:supp_loc_res_fsh}

%	\vspace*{-0.5\baselineskip}

\end{figure*}
\newpage
