# Supplementary material for: MVFNet: Multipurpose Video Forensics Network using Multiple Forms of Forensic Evidence
Source: arXiv:2503.20991 source file (2025-03-26)
Supplement: Supplementary file 6 [file supp_result_editing.tex]

\newpage
\begin{figure*}[t]
	\centering
	\includegraphics[width=1.0\linewidth]{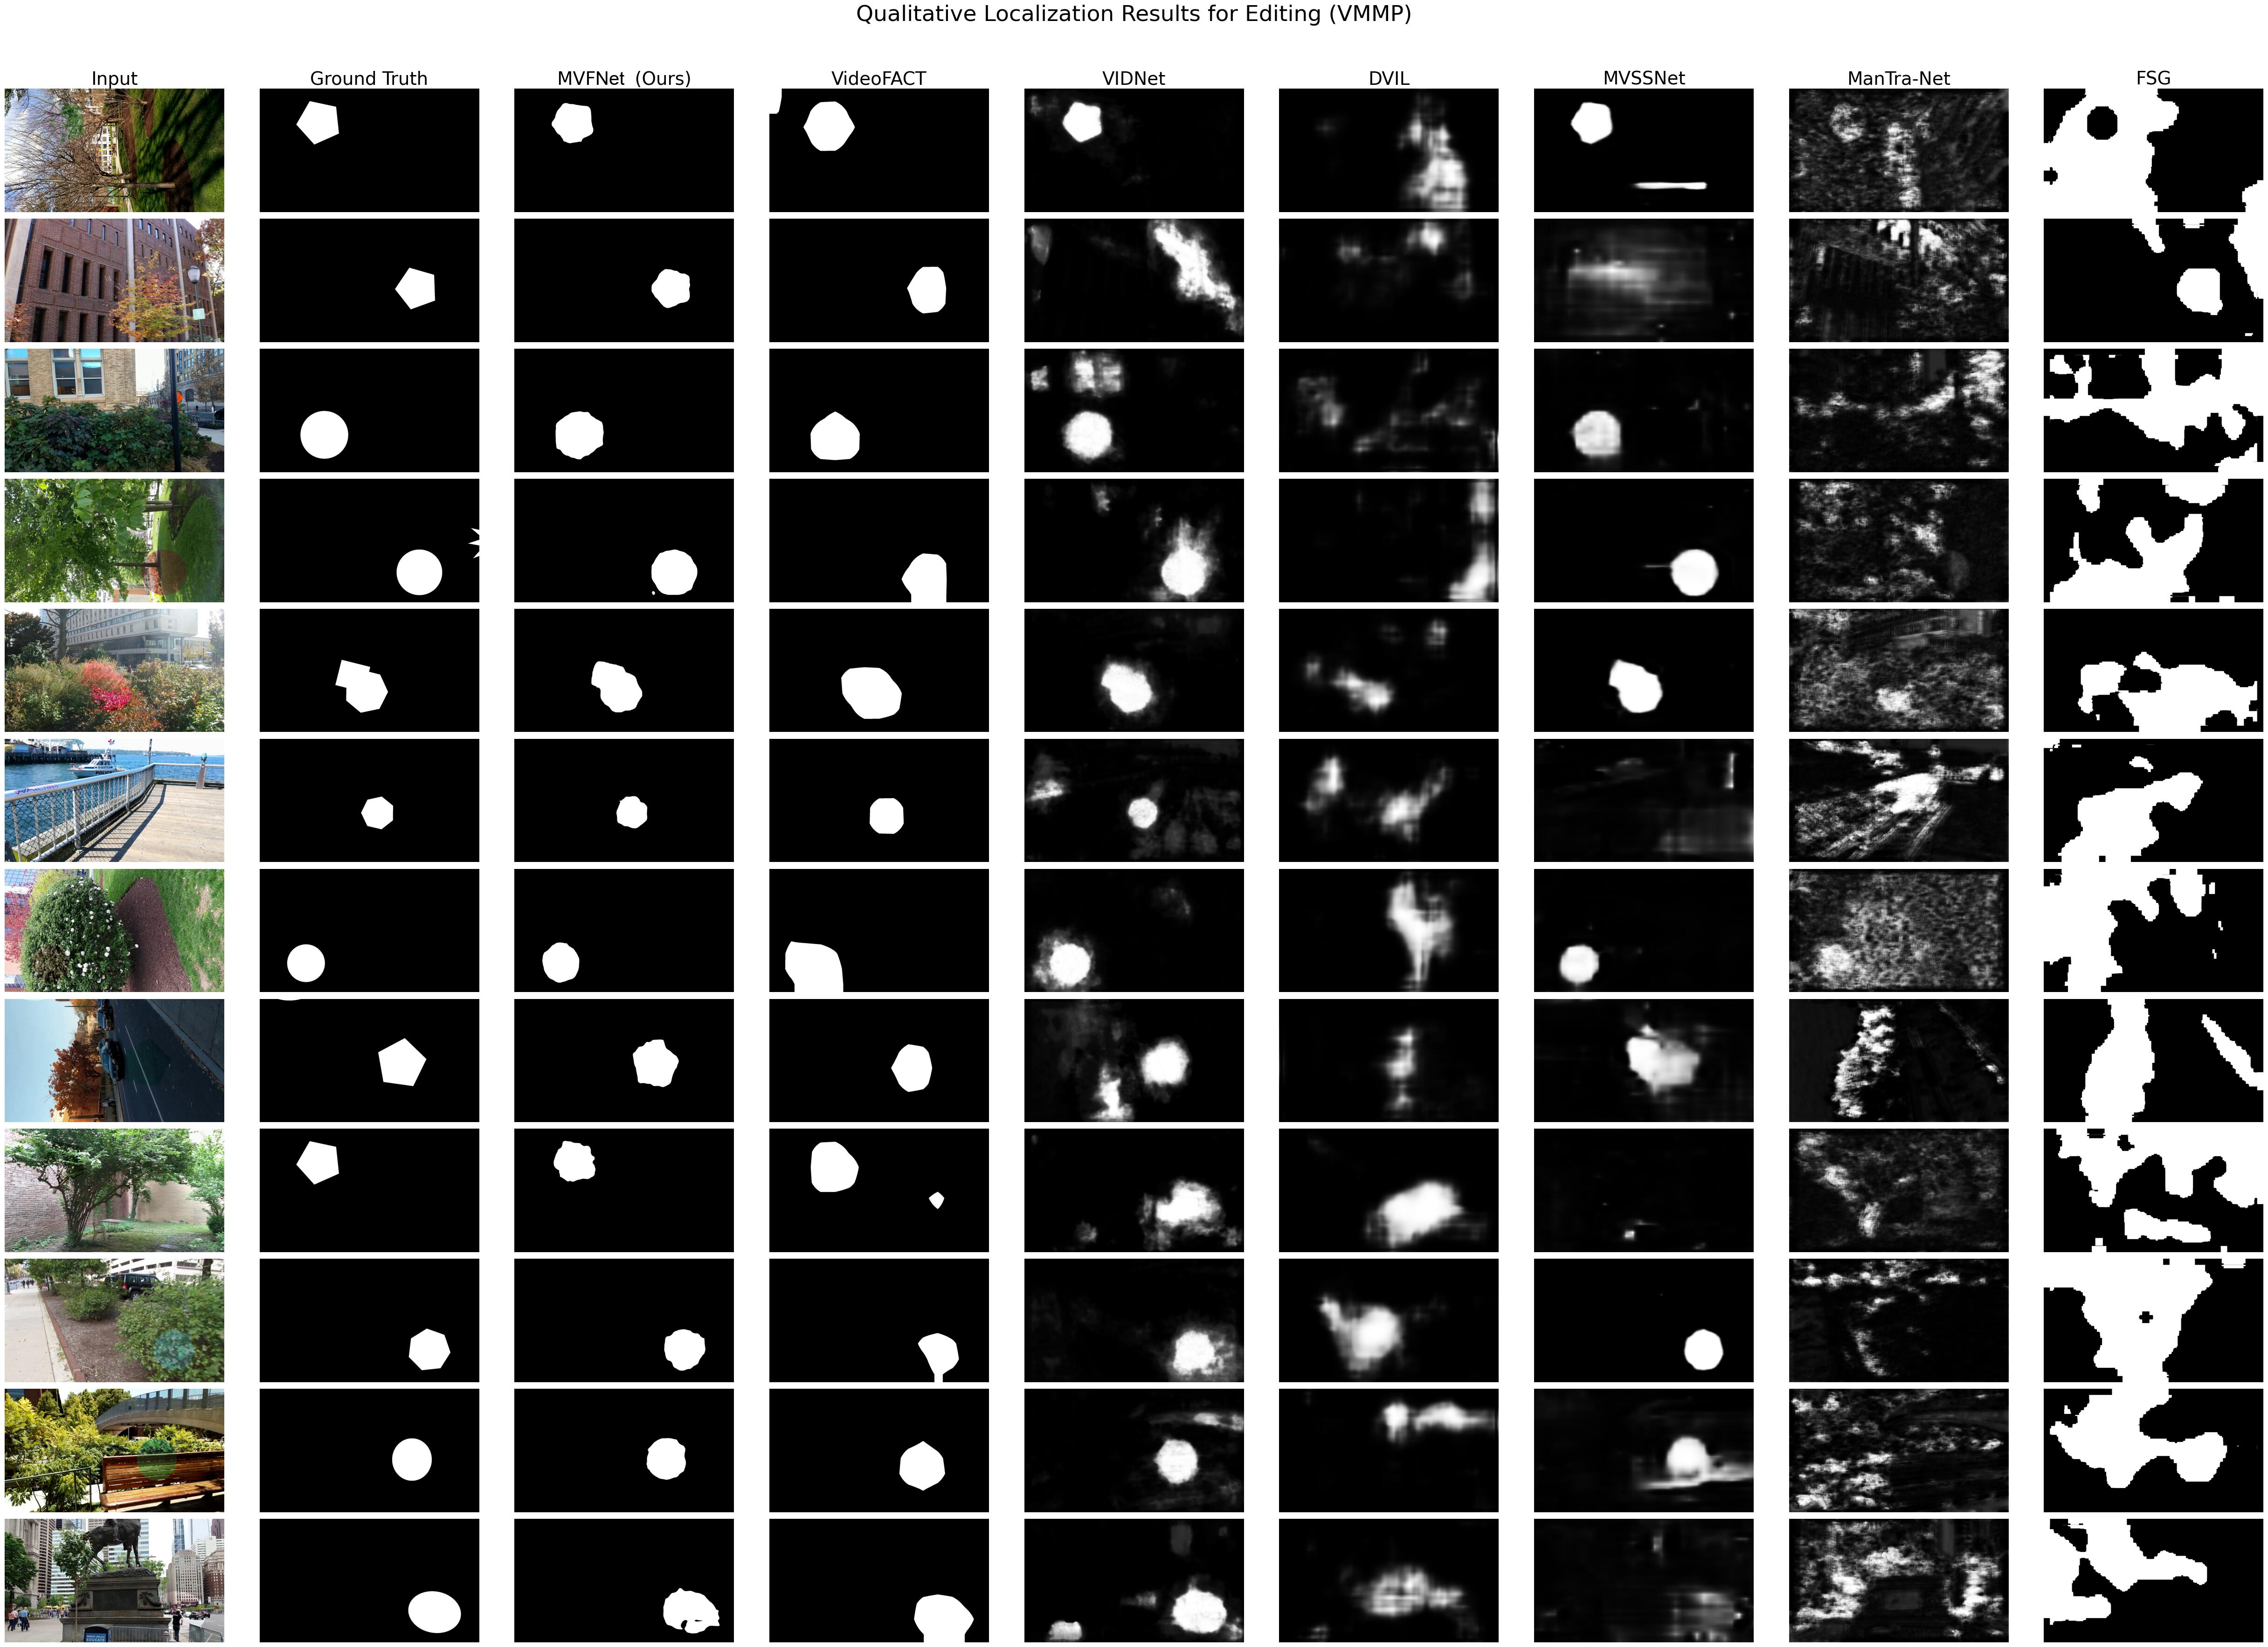}

%	\vspace*{-0.5\baselineskip}

	\caption{This figure compares the localization results for editing detection on the VMMP dataset. Our \ournetworkname method achieves the most accurate localization, closely reflecting the Ground Truth. VideoFACT shows competent localization capabilities, slightly less precise than \ournetworkname. VIDNet and DVIL, while generally effective, do not match the accuracy of VideoFACT and show a decline in performance. MVSS-Net impresses with successful localizations in the majority of cases but falls short in others. The remaining methods, ManTra-Net and FSG, largely fail to accurately localize the manipulations, with a tendency to either miss or incorrectly identify the edited regions.}

	\label{fig:supp_loc_res_editing}

%	\vspace*{-0.5\baselineskip}

\end{figure*}
\newpage
