# Supplementary material for: MVFNet: Multipurpose Video Forensics Network using Multiple Forms of Forensic Evidence
Source: arXiv:2503.20991 source file (2025-03-26)
Supplement: Supplementary file 7 [file supp_result_inpainting.tex]

\newpage
\begin{figure*}[t]
	\centering
	\includegraphics[width=1.0\linewidth]{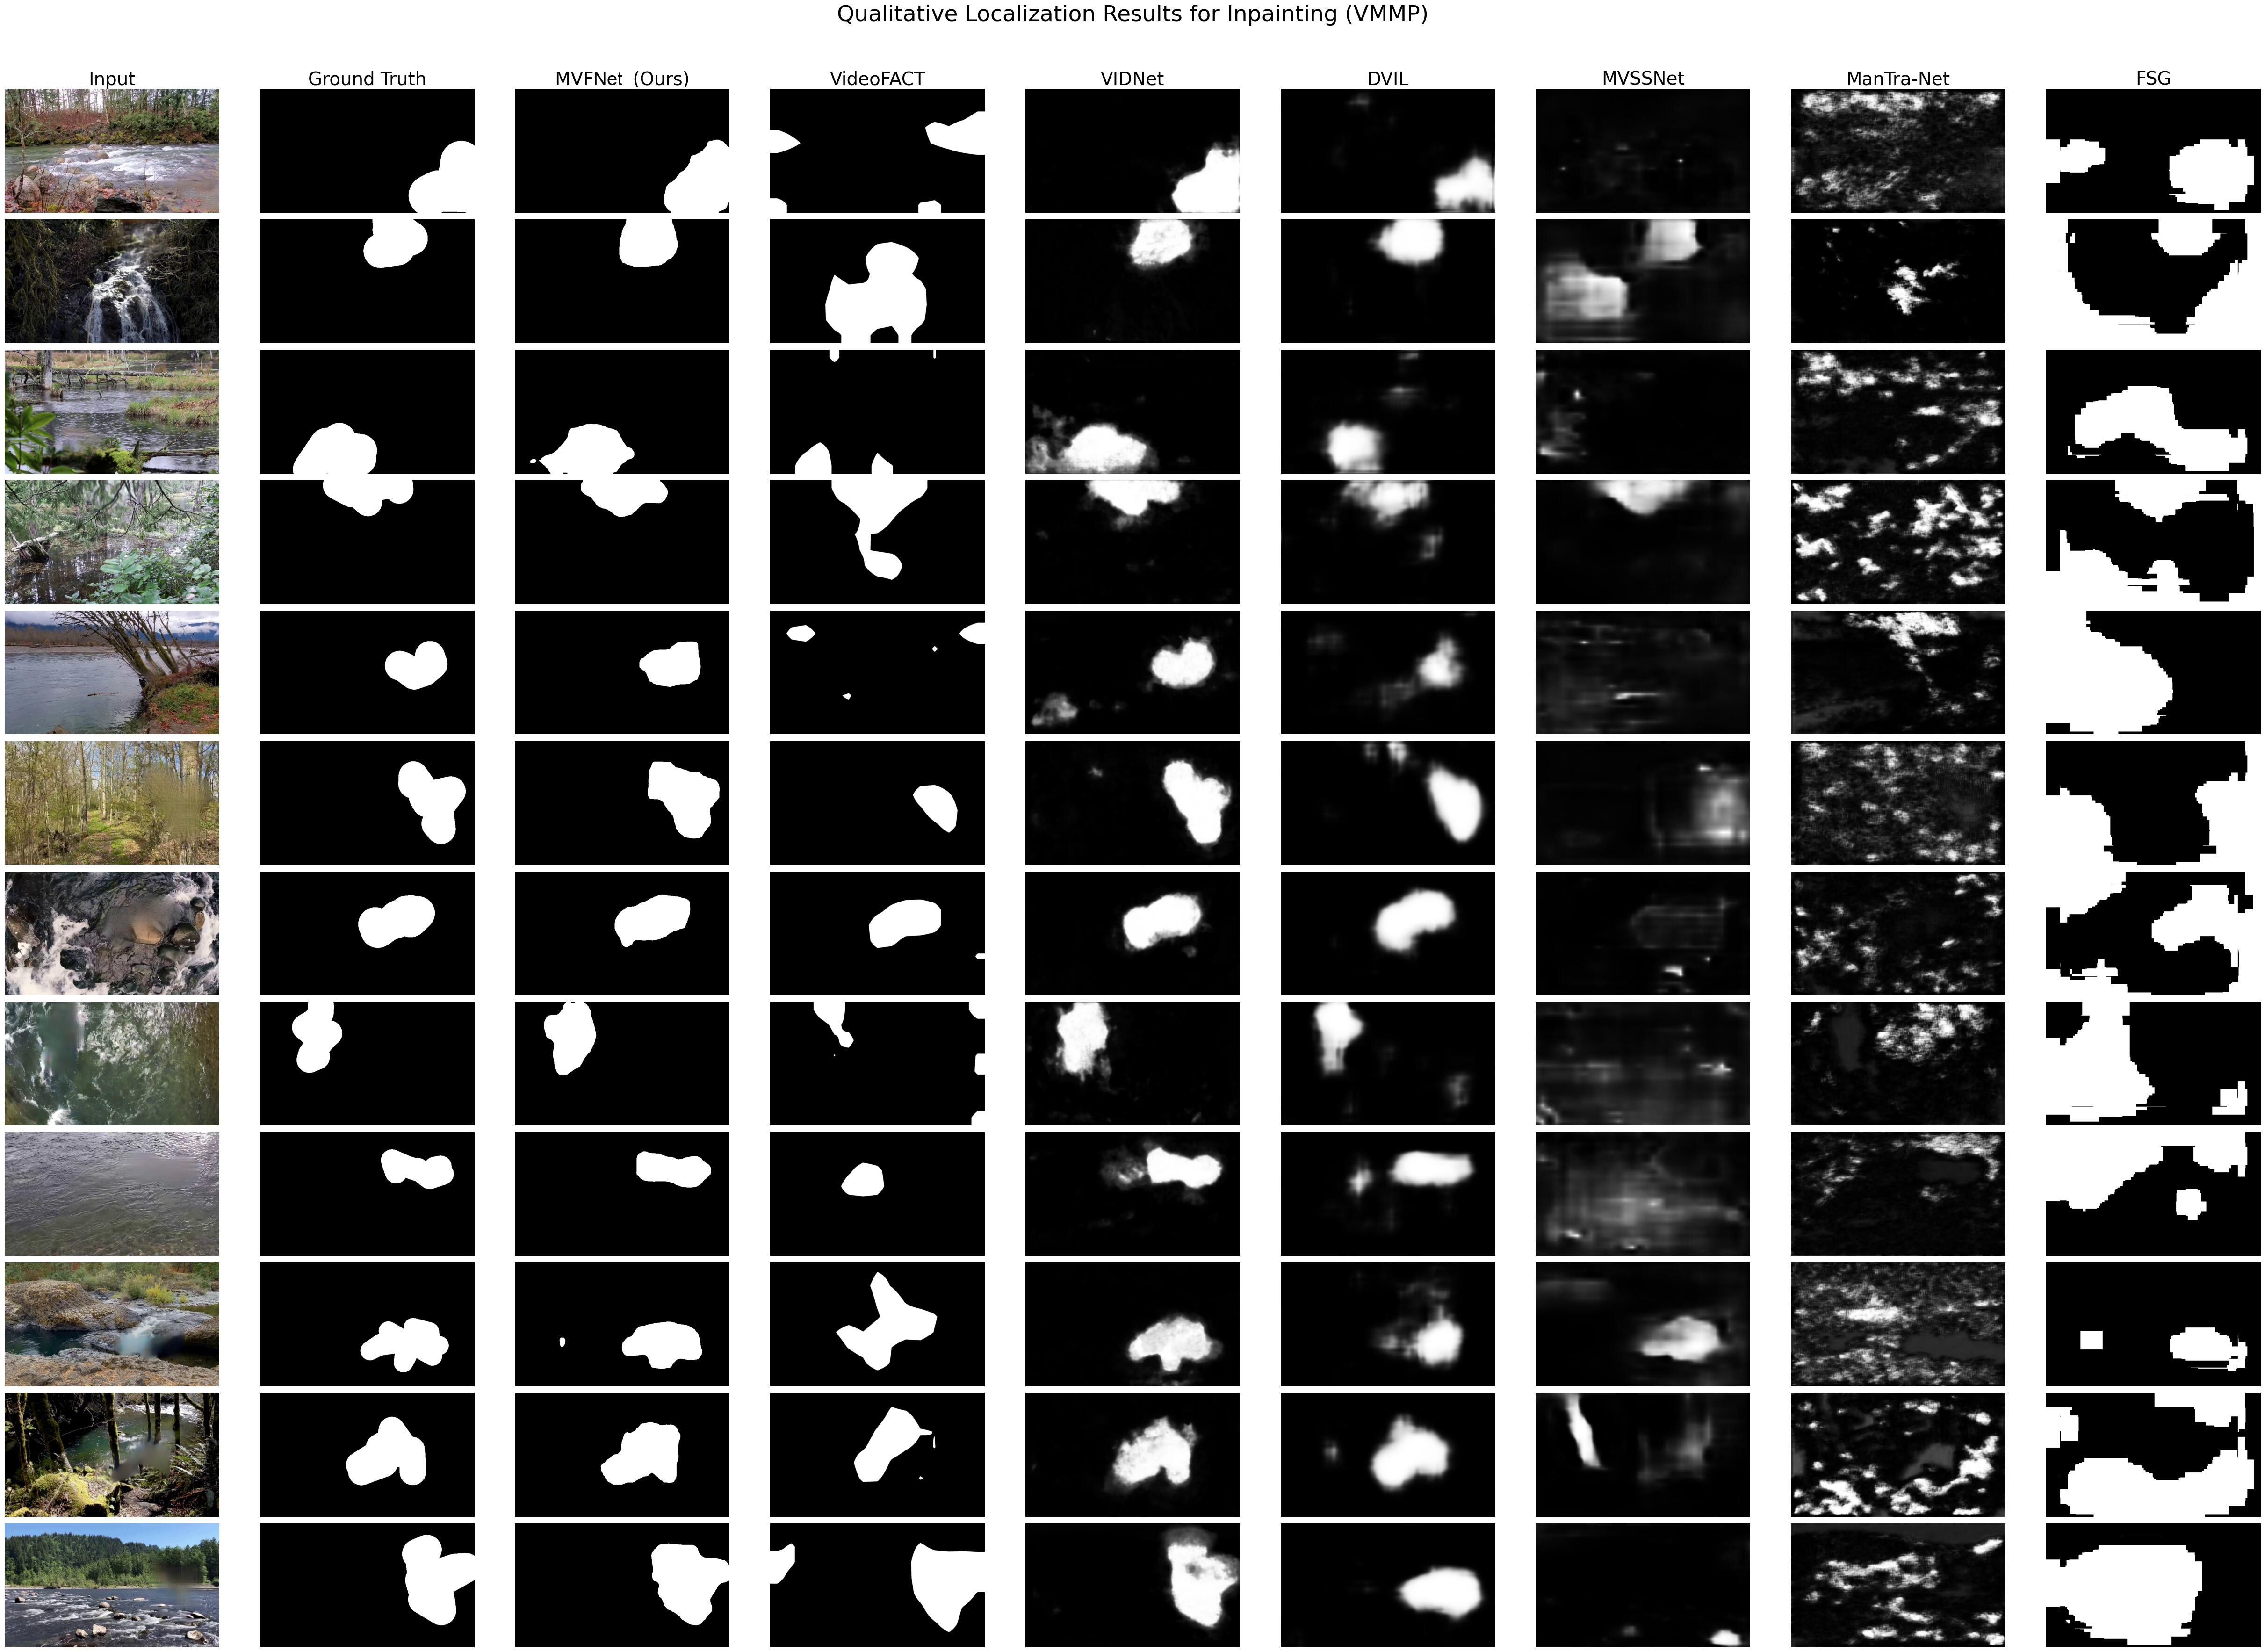}

%	\vspace*{-0.5\baselineskip}

	\caption{This figure presents localization results from various methods for an inpainting detection challenge. Our \ournetworkname method exhibits accurate and consistent localization closely mirroring the Ground Truth. VideoFACT achieves decent results, albeit with less precision than \ournetworkname. Both VIDNet and DVIL demonstrate good performance, delivering results that are on-par with our method in terms of accuracy. Conversely, MVSS-Net, ManTra-Net, and FSG struggle to identify the manipulated areas correctly, frequently misplacing the localization or entirely missing the inpainted regions.}

	\label{fig:supp_loc_res_inpainting}

%	\vspace*{-0.5\baselineskip}

\end{figure*}
\newpage
