# Supplementary material for: MVFNet: Multipurpose Video Forensics Network using Multiple Forms of Forensic Evidence
Source: arXiv:2503.20991 source file (2025-03-26)
Supplement: Supplementary file 8 [file supp_result_inpainting_e2fgvi.tex]

\newpage
\begin{figure*}[t]
	\centering
	\includegraphics[width=1.0\linewidth]{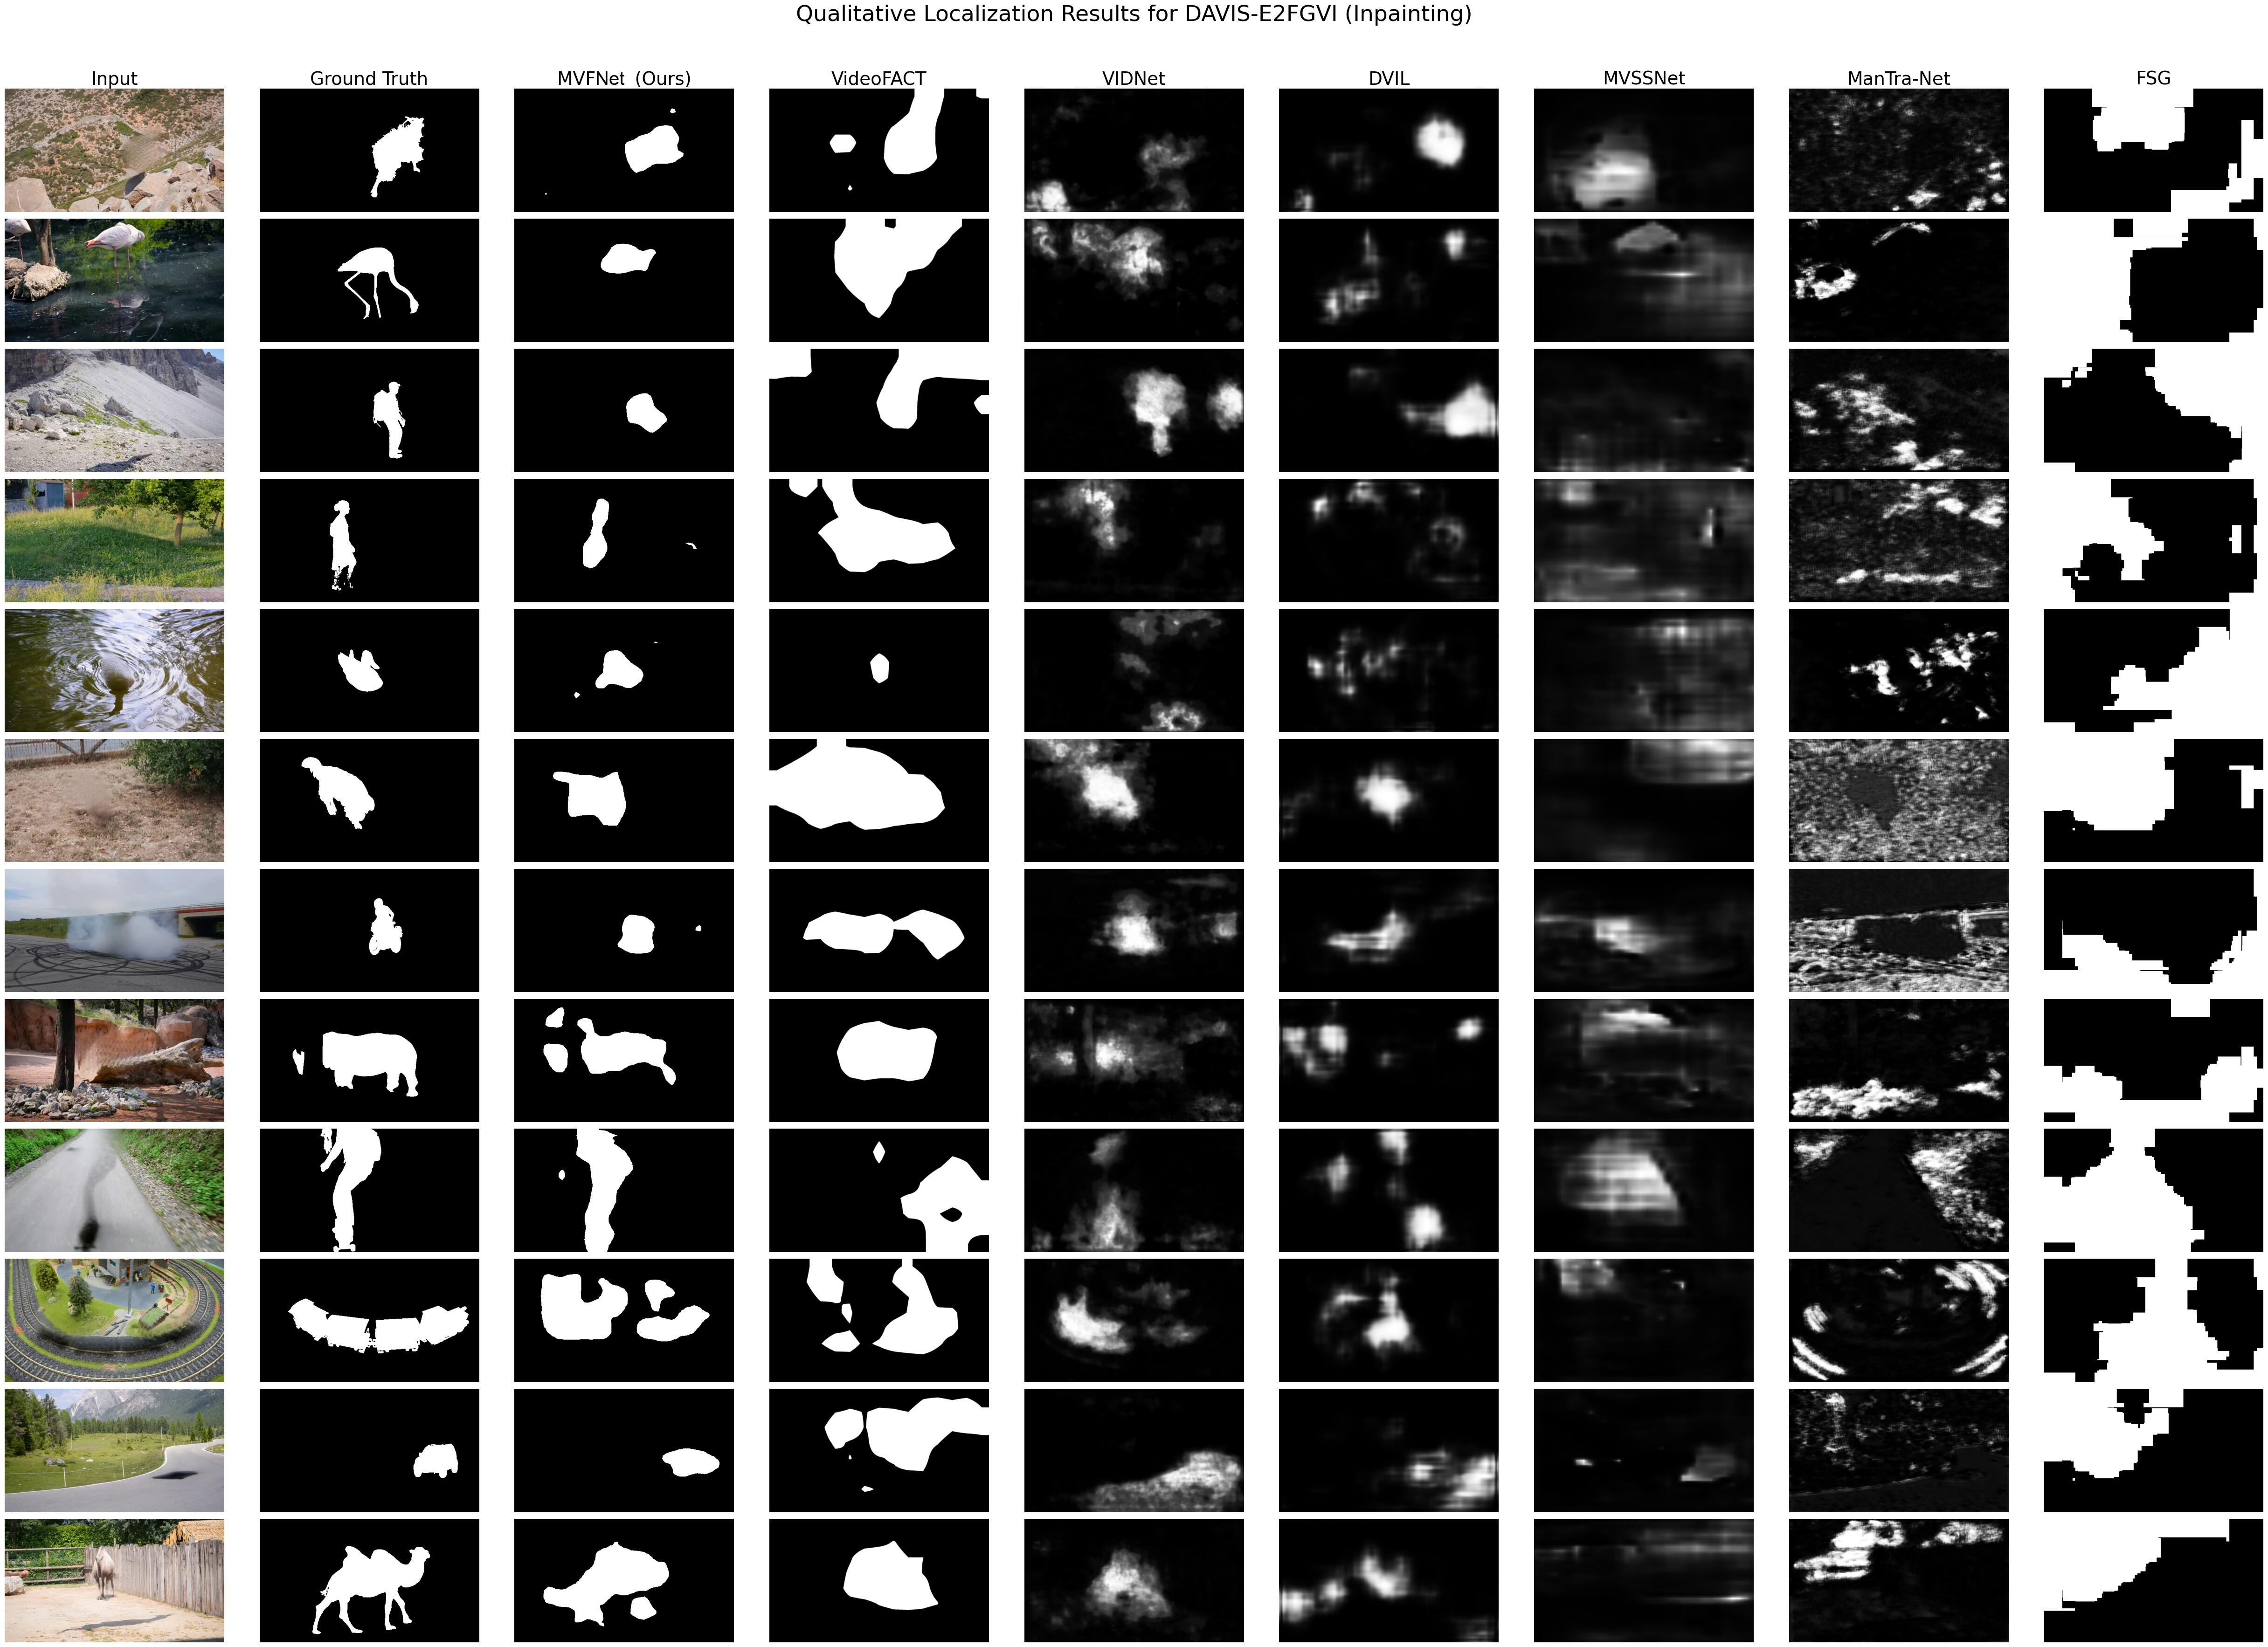}

	\vspace*{-0.5\baselineskip}

	\caption{This figure displays localization results for inpainting detection on the DAVIS-E2FGVI dataset. Our \ournetworkname approach outperforms others by producing localization masks that closely match the Ground Truth, with high precision and minimal false detections. VIDNet and DVIL demonstrate reasonable accuracy, effectively capturing the manipulated regions with some minor imprecisions. VideoFACT, while detecting the general area of manipulation, tends to generate overly broad masks, leading to a significant amount of false positives. The results from MVSS-Net, ManTra-Net, and FSG show a marked lack of accuracy, failing to provide useful localization in most cases and indicating a substantial departure from the Ground Truth.}

	\label{fig:supp_loc_res_e2fgvi}

	\vspace*{-0.5\baselineskip}

\end{figure*}
\newpage
