# Supplementary material for: MVFNet: Multipurpose Video Forensics Network using Multiple Forms of Forensic Evidence
Source: arXiv:2503.20991 source file (2025-03-26)
Supplement: Supplementary file 9 [file supp_result_inpainting_fuseformer.tex]

\newpage
\begin{figure*}[t]
	\centering
	\includegraphics[width=1.0\linewidth]{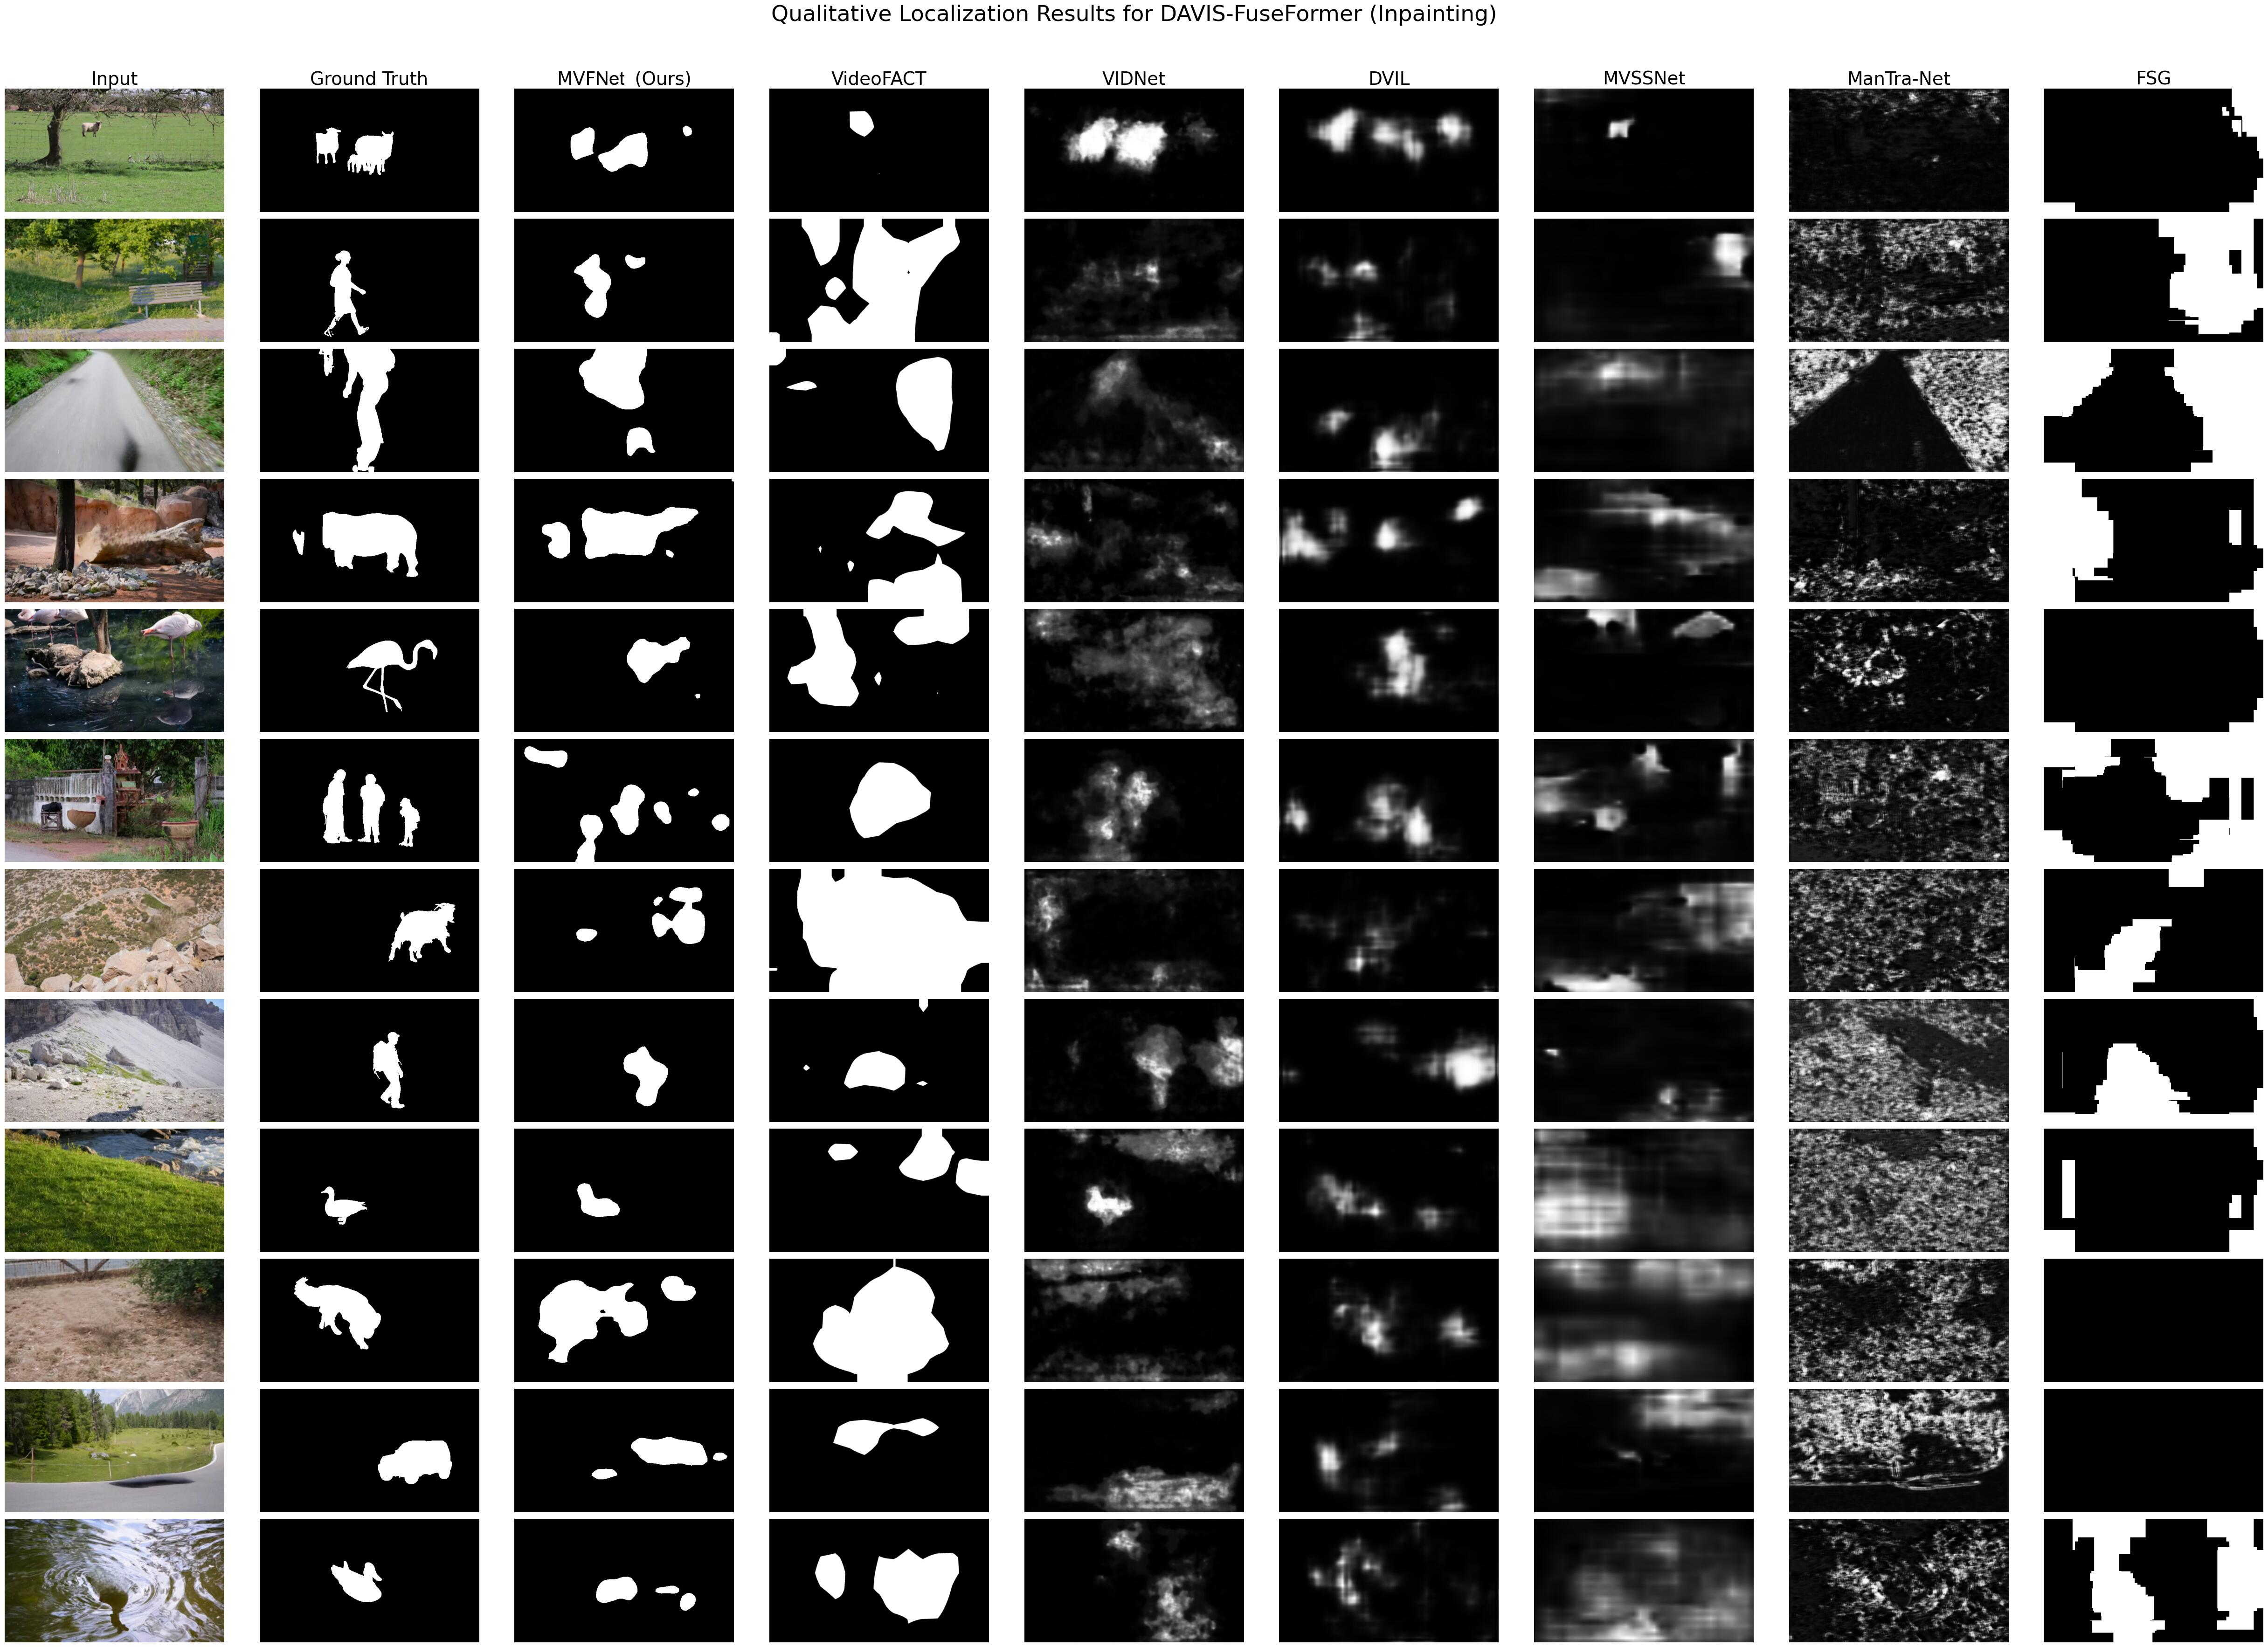}

%	\vspace*{-0.5\baselineskip}

	\caption{Localization results for inpainting detection on the DAVIS-FuseFormer dataset are compared across various methods. The \ournetworkname approach, our proposed method, consistently yields localization masks that are tightly aligned with the Ground Truth, demonstrating high fidelity and specificity. VideoFACT, while identifying the area of manipulation, tends to overextend the localization boundaries beyond the actual region. VIDNet shows a moderate level of accuracy, capturing significant portions of the manipulated areas but with less precision. DVIL, although somewhat effective, produces inconsistent results with varying degrees of overgeneralization. MVSS-Net, ManTra-Net, and FSG exhibit poor performance, with ManTra-Net and FSG generating particularly extensive and inaccurate localizations that deviate significantly from the Ground Truth.}

	\label{fig:supp_loc_res_fuseformer}

%	\vspace*{-0.5\baselineskip}

\end{figure*}
\newpage
