# Supplementary material for: MVFNet: Multipurpose Video Forensics Network using Multiple Forms of Forensic Evidence
Source: arXiv:2503.20991 source file (2025-03-26)
Supplement: Supplementary file 10 [file supp_result_splicing.tex]

\newpage
\begin{figure*}[t]
	\centering
	\includegraphics[width=1.0\linewidth]{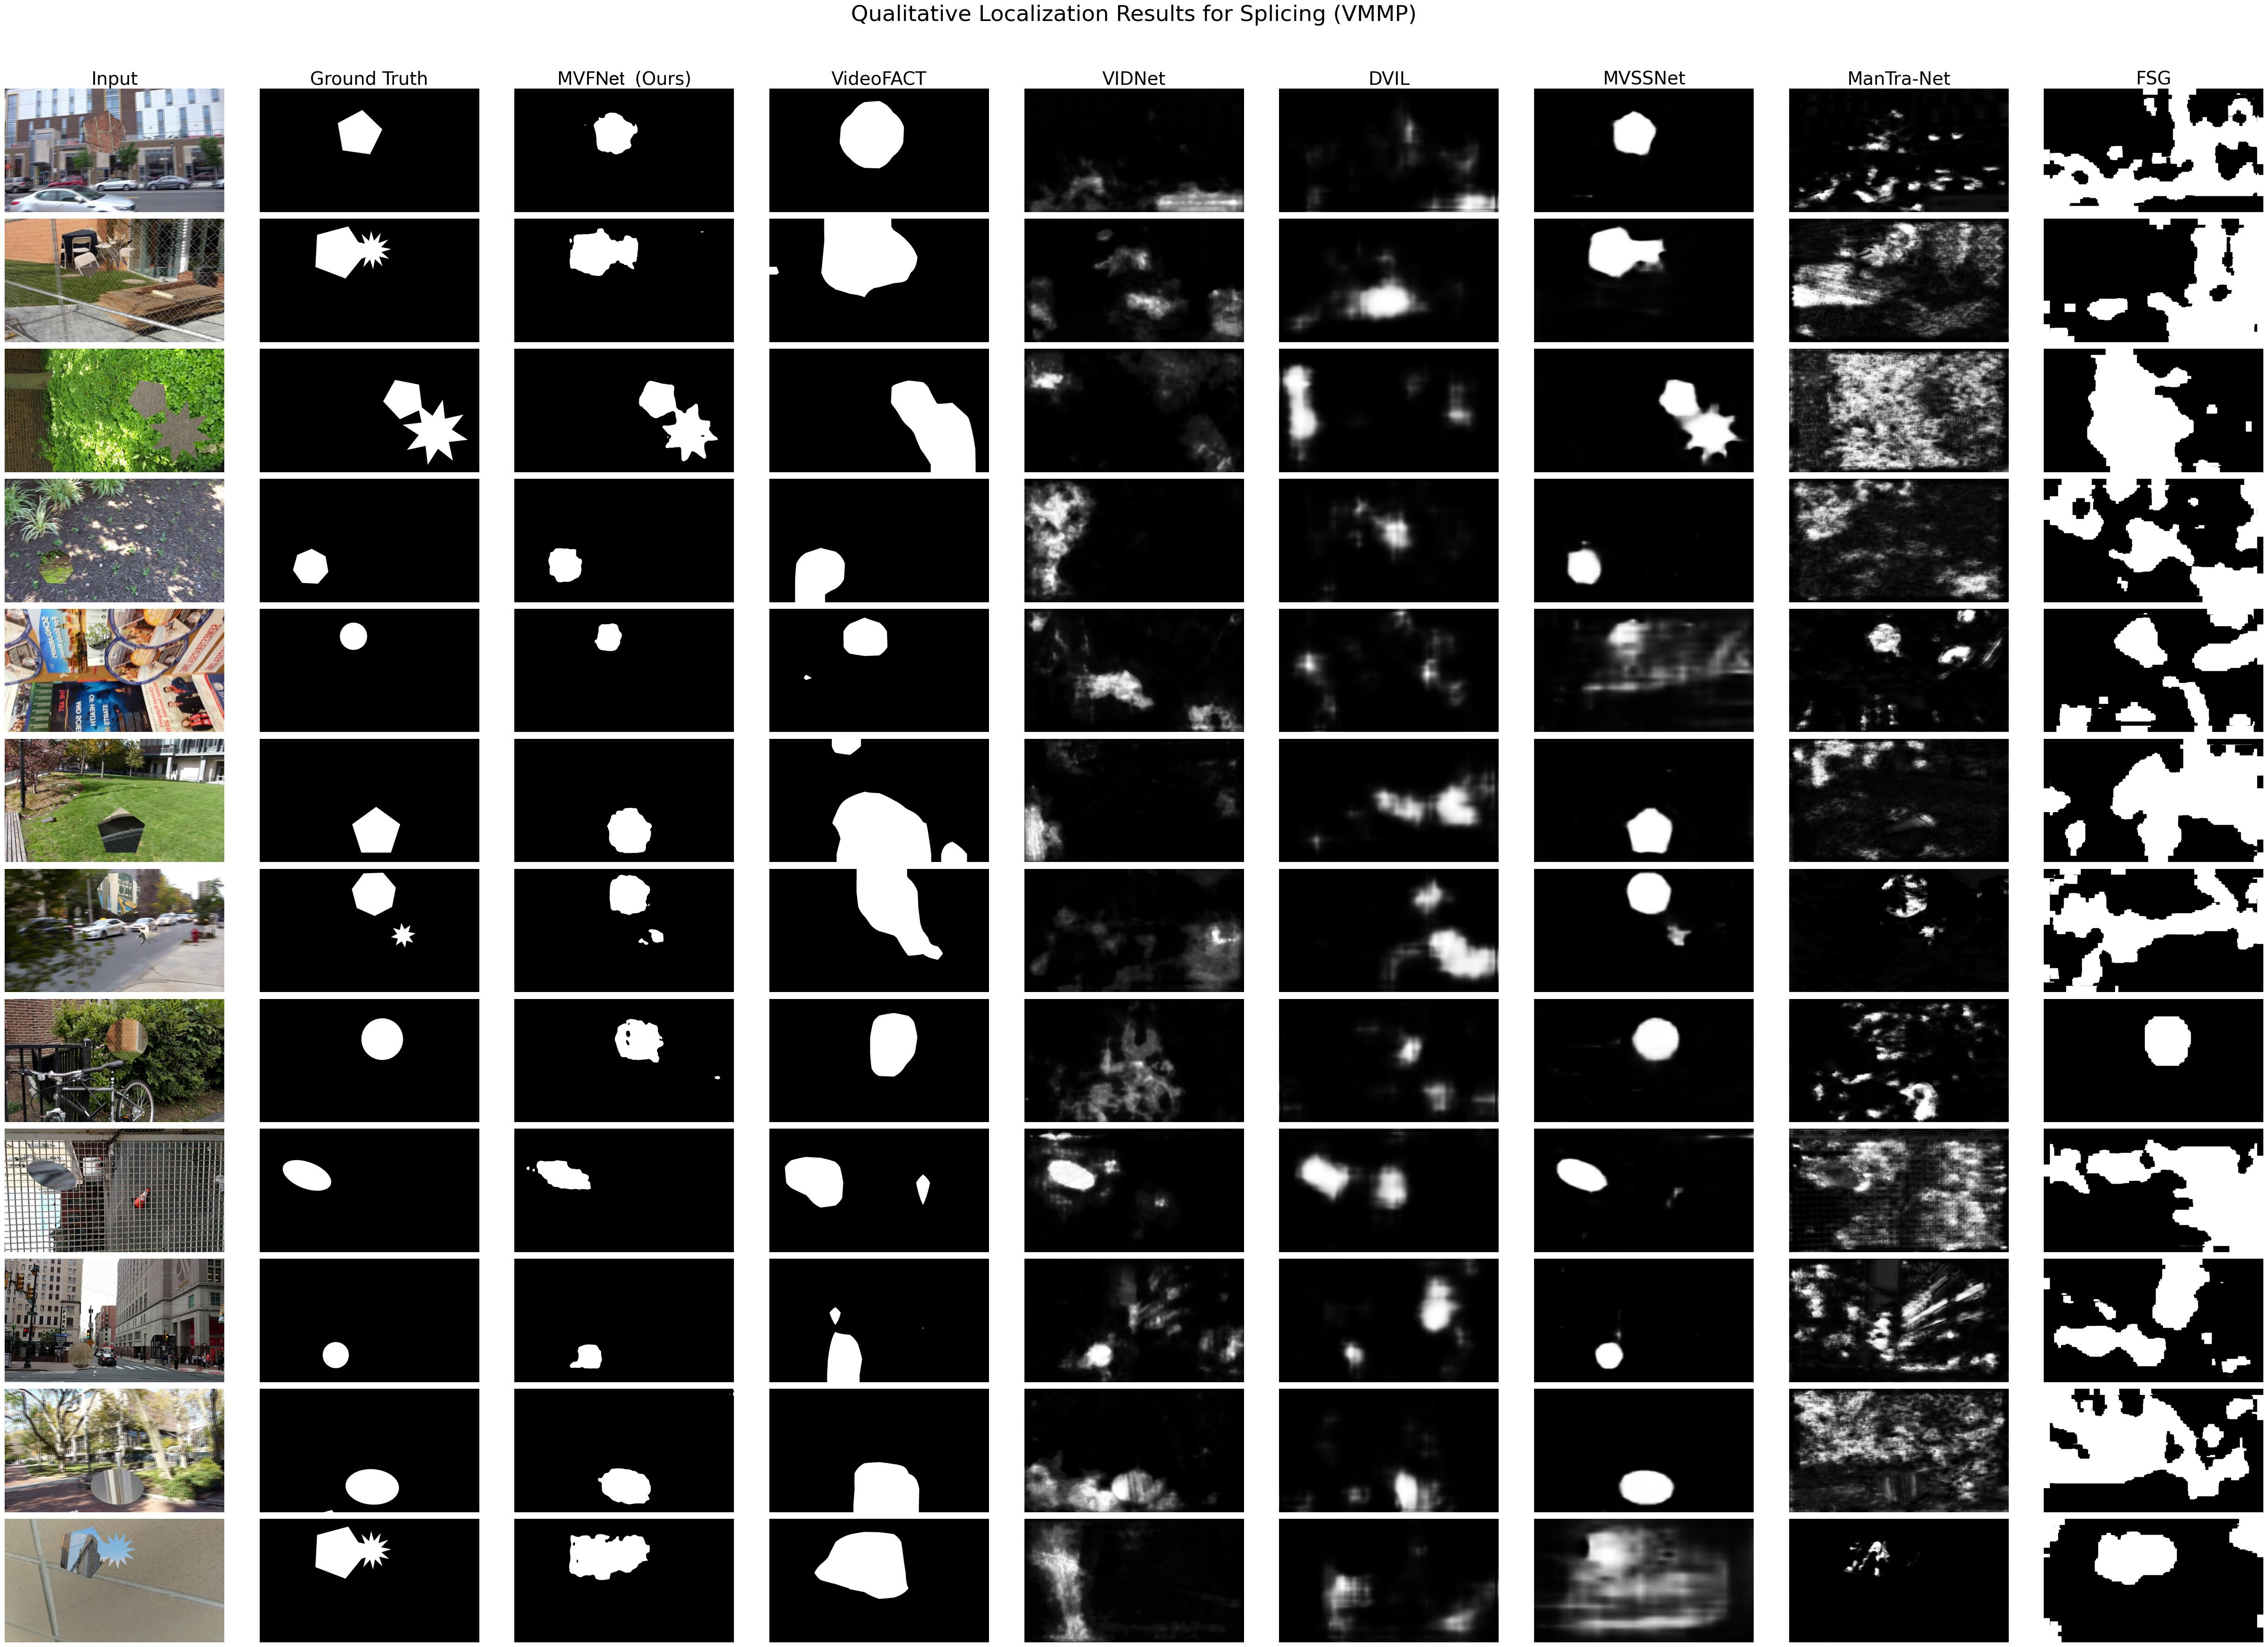}

%	\vspace*{-0.5\baselineskip}

	\caption{Localization accuracy for splicing detection is evaluated across different methods on the VMMP dataset. \ournetworkname showcases a high degree of precision, closely matching the Ground Truth. VideoFACT, while reasonably effective, does not attain the same level of accuracy as \ournetworkname. VIDNet and DVIL display less precision compared to VideoFACT, with their performance varying across different cases. MVSS-Net excels in a majority of scenarios but sometimes fails to detect the manipulation entirely. ManTra-Net and FSG generally provide inaccurate localizations, often identifying incorrect regions or missing the splicing altogether.}

	\label{fig:supp_loc_res_splicing}

%	\vspace*{-0.5\baselineskip}

\end{figure*}
\newpage
