# Supplementary material for: MVFNet: Multipurpose Video Forensics Network using Multiple Forms of Forensic Evidence
Source: arXiv:2503.20991 source file (2025-03-26)
Supplement: Supplementary file 11 [file supp_result_videosham.tex]

\newpage
\begin{figure*}[t]
	\centering
	\includegraphics[width=1.0\linewidth]{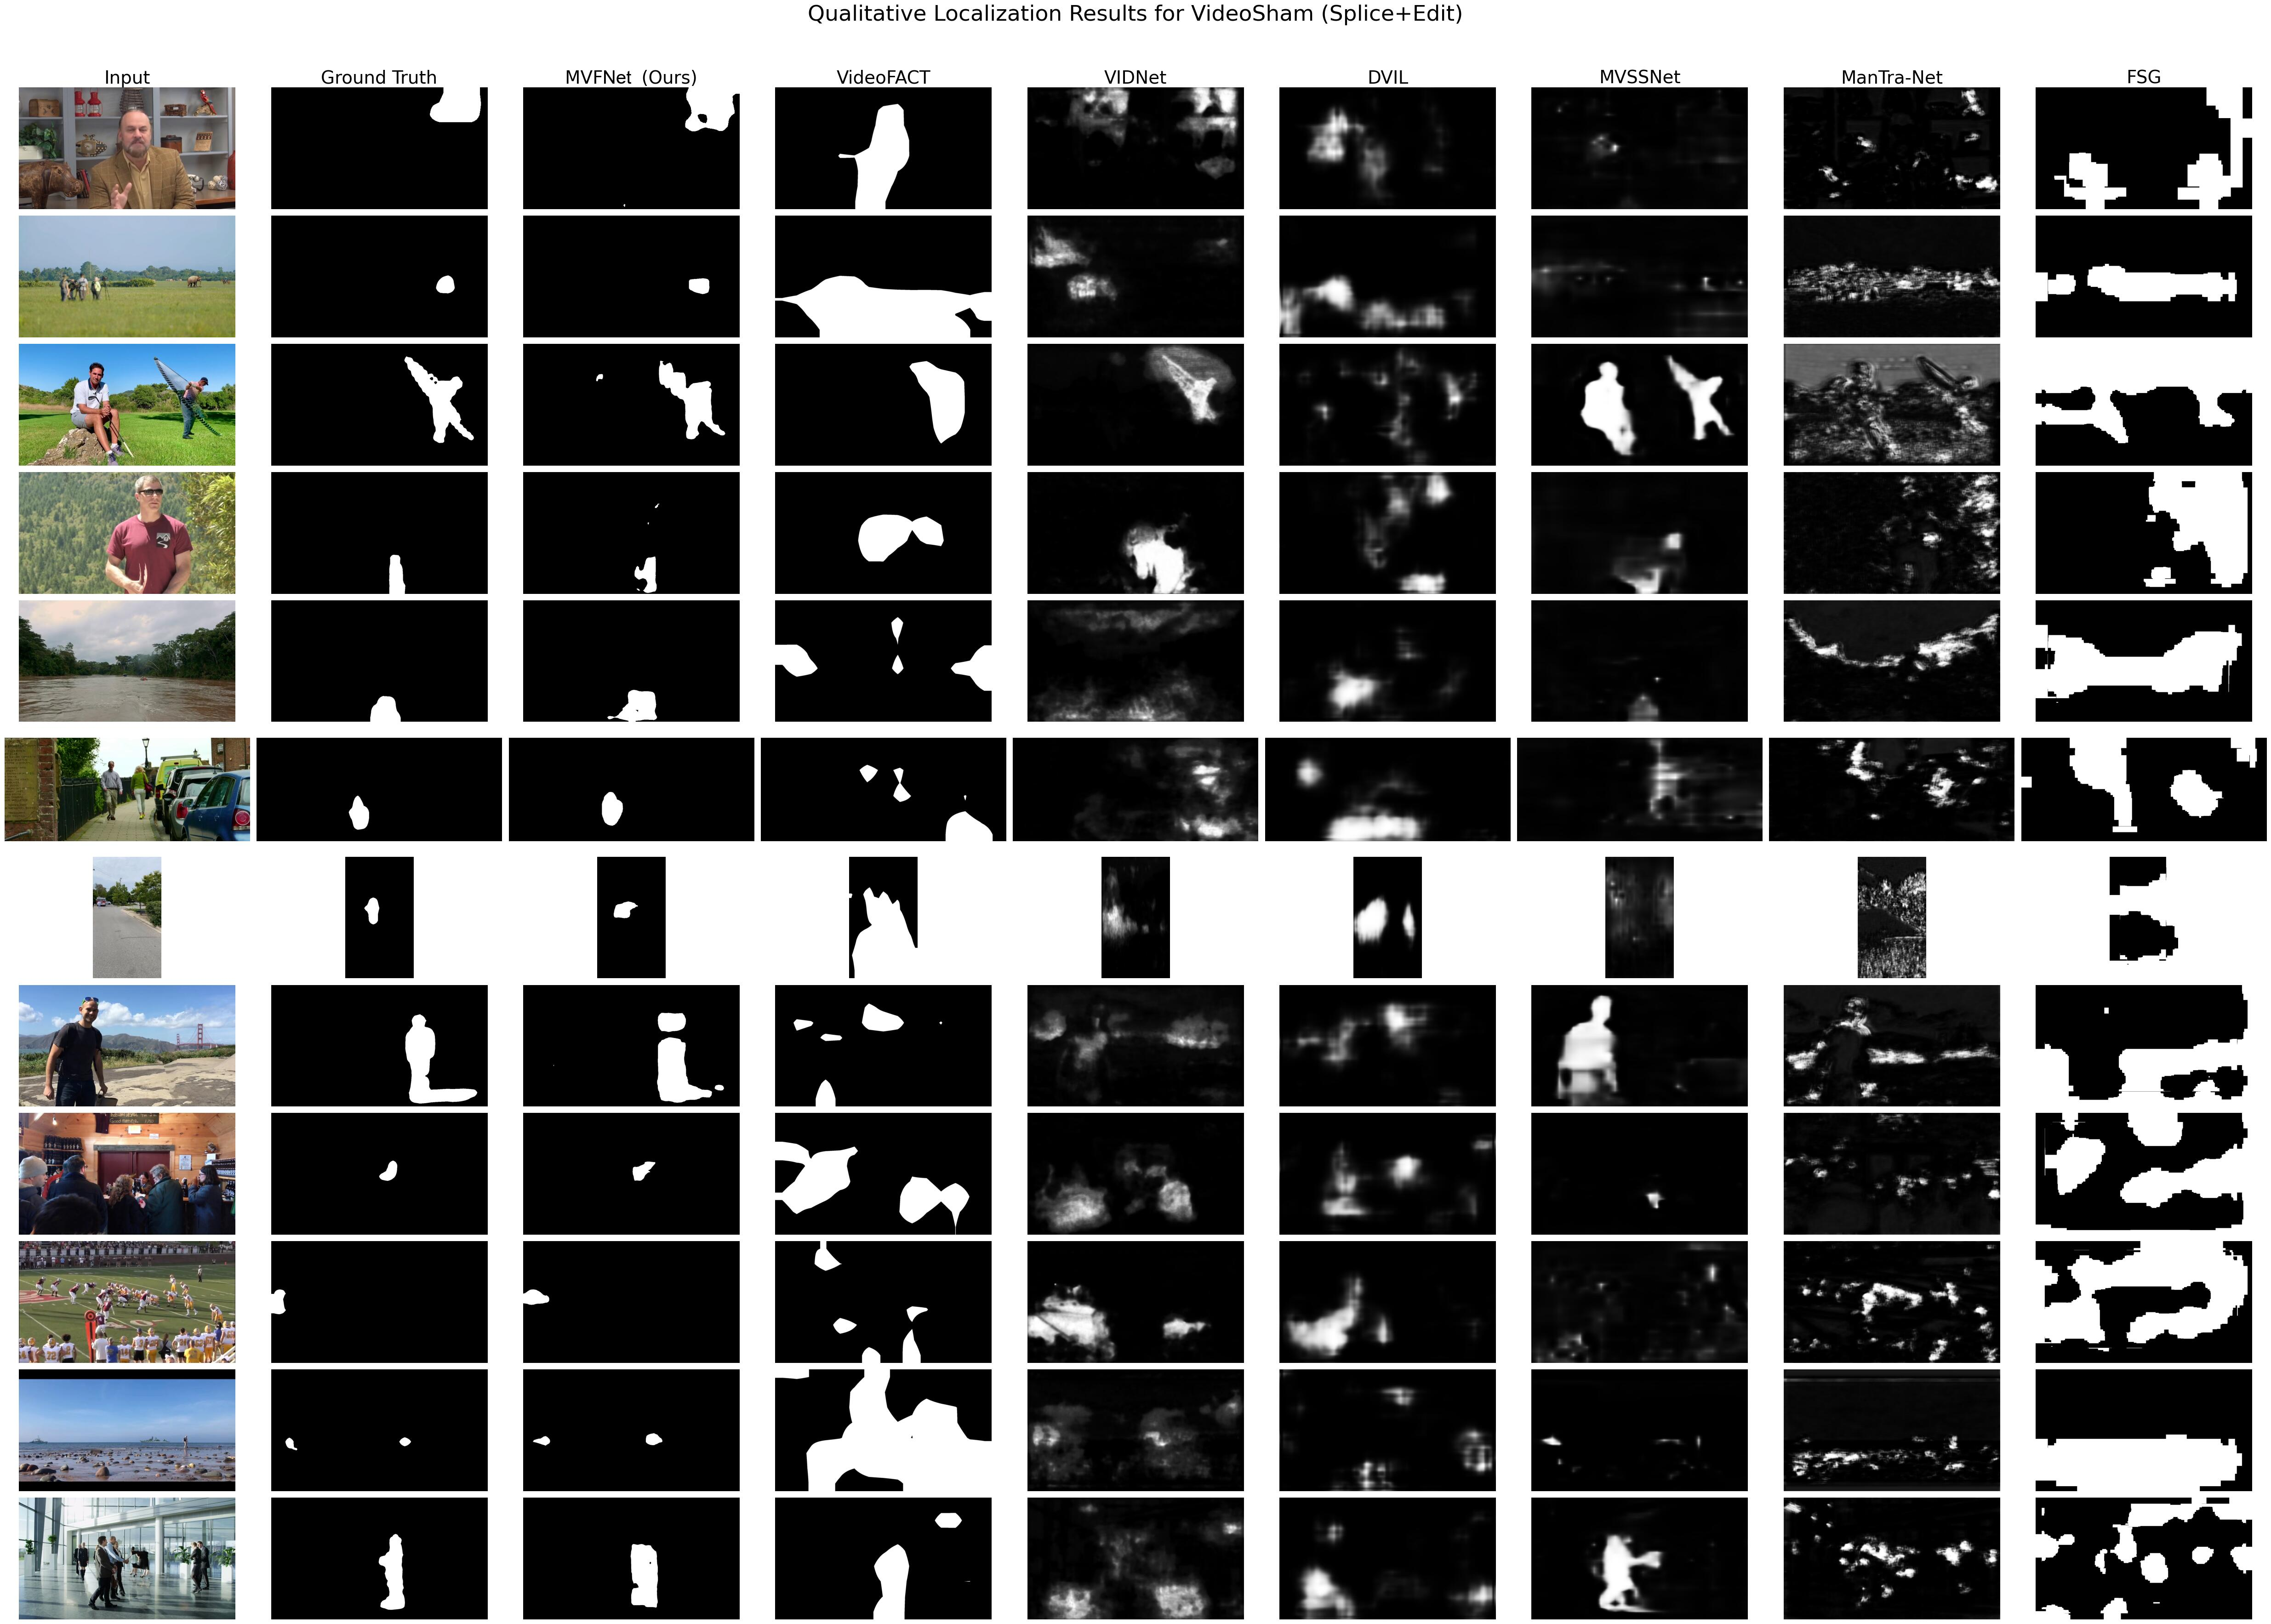}

%	\vspace*{-0.5\baselineskip}

	\caption{Comparative localization results for video manipulation detection on the Adobe VideoSham dataset (Splice+Edit). The Ground Truth column displays the actual manipulated areas, followed by the detection results from our method (\ournetworkname) and other leading approaches: VideoFACT, VIDNet, DVIL, MVSS-Net, ManTra-Net, and FSG. Our method demonstrates superior localization precision, closely mirroring the Ground Truth, with clear, well-defined boundaries and minimal false positives. VideoFACT and VIDNet exhibit moderate localization accuracy but with less distinct boundaries. DVIL and MVSS-Net present overgeneralized localizations with significant false positives, while ManTra-Net and FSG show mostly inaccurate detections.}

	\label{fig:supp_loc_res_videosham}

%	\vspace*{-0.5\baselineskip}

\end{figure*}
\newpage
