# Supplementary material for: MVFNet: Multipurpose Video Forensics Network using Multiple Forms of Forensic Evidence
Source: arXiv:2503.20991 source file (2025-03-26)
Supplement: Supplementary file 12 [file Supp_FFE.tex]

\section{Details on Spatial Forensic Residual Feature Extractor}

Here we provide more details about the architecture of the Spatial Forensic Residual Feature Extractor. The system diagram for this subnetwork can be found in Fig.~\ref{fig:ffe_arch}. As stated in Sec. 3.1, we first create a rich set of learned forensic residuals using a constrained convolutional layer proposed in~\cite{MISLnet}. Then, these residuals are analyzed using a series of fused inverted residual (FIR) blocks~\cite{MobileNetV2} with specifications shown in Fig.~\ref{fig:ffe_arch}. In general, the number of embedding dimension increases (24 $\rightarrow$ 48 $\rightarrow$ 64 $\rightarrow$ 128 $\rightarrow$ 256) and the input dimension is subsequently reduced by a total factor of 8.

\begin{figure*}[!h]
	\pullup
	\centering
	\includegraphics[width=1.0\linewidth]{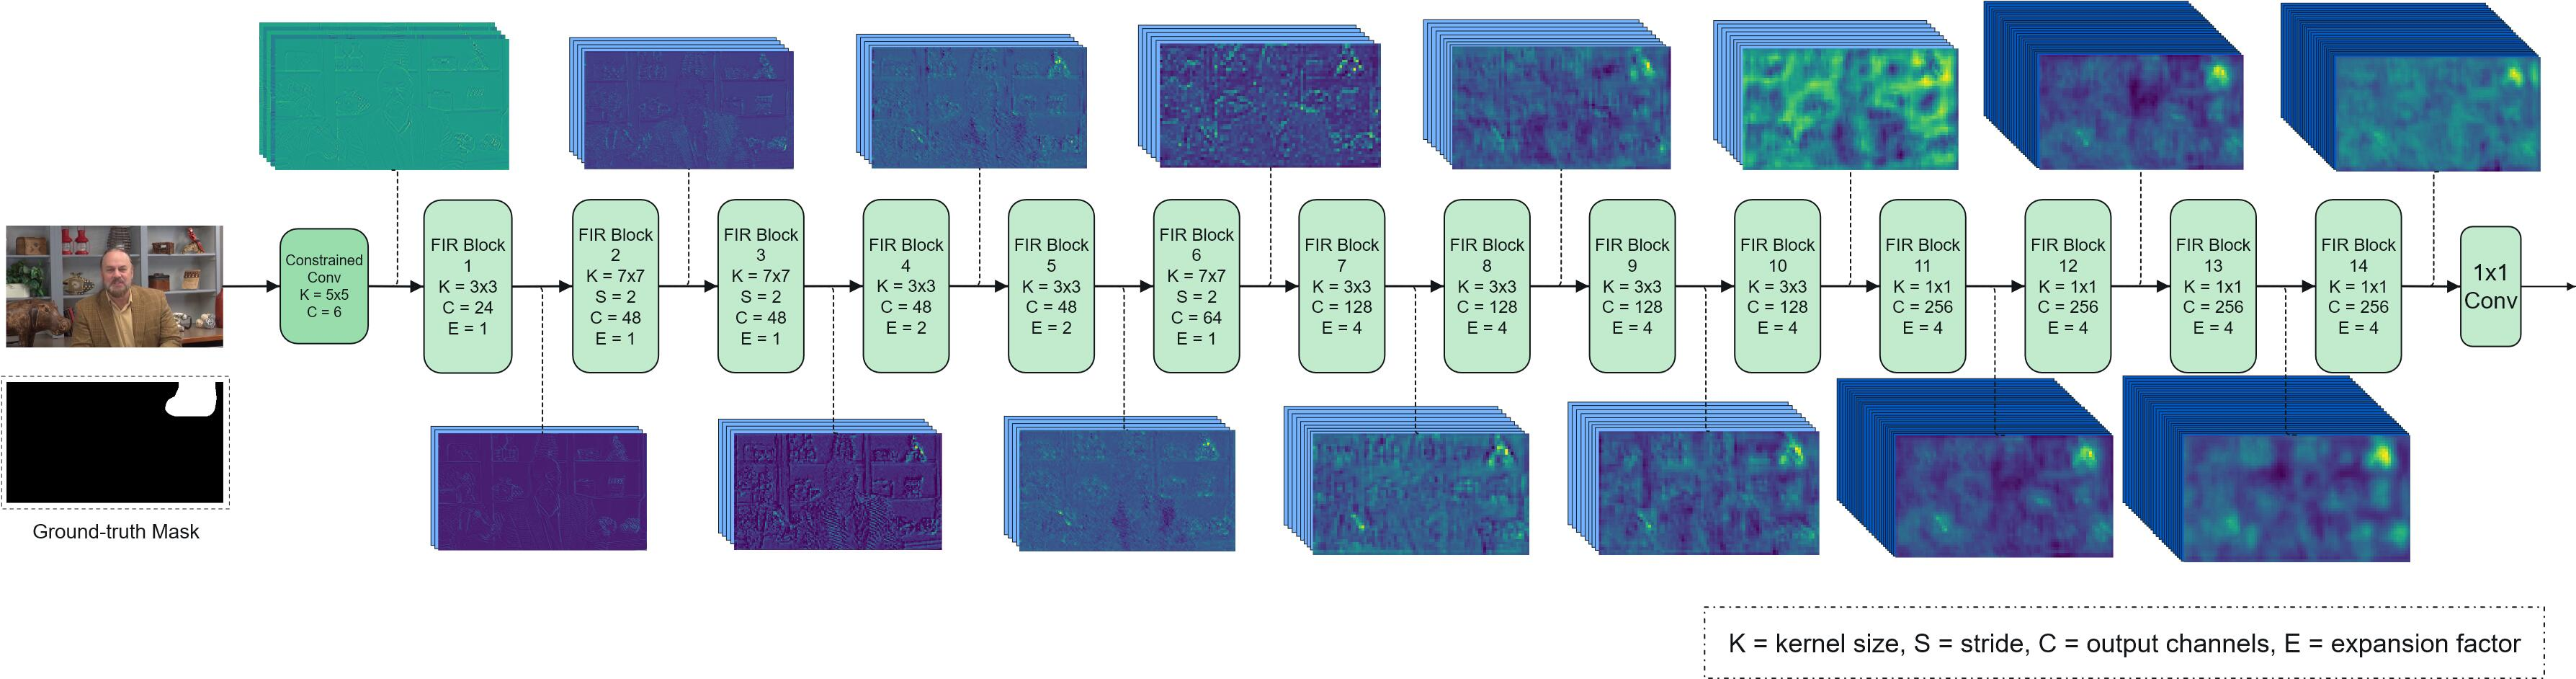}
	\caption{This figure shows the details of the Spatial Forensic Residual Feature Extractor.}
	\label{fig:ffe_arch}
	\pullupp
\end{figure*}

\section{Details on Temporal Forensic Residual Feature Extractor}
\label{supp:TRFE}

The temporal residual forensic features are also extracted using a residual extractor and series of FIR blocks. Here, the focus is on extracting low-level pixel-intensity-related features that when taken the difference between adjacent frames, reveals temporal inconsistencies. This process starts with the RGB input frame undergoing a shallow residually connected convolutional layer, which is succeeded by an array of convolutional, normalization, and SiLU activation layers to compress the dimensionality of the input while modestly amplify the feature set. Subsequent to this dimensionality reduction, the extracted low-level residuals are fed through a series of 4 FIR blocks, with the number of embedding dimension increases from 8 $\rightarrow$ 16 $\rightarrow$ 32 $\rightarrow$ 64, and the input dimension is reduced by a total factor of 8.
