# Supplementary material for: MVFNet: Multipurpose Video Forensics Network using Multiple Forms of Forensic Evidence
Source: arXiv:2503.20991 source file (2025-03-26)
Supplement: Supplementary file 13 [file Supp_FFE_Pretraining_v1.tex]

\section{Spatial Forensic Residual Feature Extractor Pretraining}
\label{supp:FRFE_pretrain}

In order to pre-train the Spatial Forensic Residual Feature Extractor in our network, we developed a novel pre-training strategy. Here, we build upon prior approaches used in many multimedia forensic methods, in which forensic embeddings are learned by pre-training a network to perform forensic camera model identification (i.e. determining which camera model was used to capture an image)~\cite{MISLnet, EXIFnet, Noiseprint, FSG, FSM}.
Unlike prior work~\cite{VideoFACT, MISLnet, EXIFnet, Noiseprint, FSG, FSM}, however, our network does not produce a single embedding. Instead, it produces a high dimensional feature set which is subsequently pooled into several embeddings across multiple scales. As a result, existing forensic pre-training approaches cannot be used in our network.

Our pre-training strategy requires the high dimensional features produced by our module to produce camera model identification results that are both accurate and consistent across multiple spatial scales. To accomplish this, we create a multi-headed pre-training network in which the output of the spatial forensic residual feature extractor is passed through our multi-scale pooling module to produce localized embeddings across multiple scales. Each embedding is then passed to an classification head, which produces an output camera model identification likelihood $\theta_{i,j}^{k,c}$ for camera model $c$, where $i$ and $j$ denote the spatial index of the embedding at scale $k$. These multi-scale, spatially distributed decisions are then aggregated and used to produce an overall pre-training loss:

\begin{equation}
	\mathcal{L}_{\text{F}} = \sum_{k} \frac{-\lambda_k}{2^{2k}} \sum_{i,j} \sum_{c}
	\log\left(\frac{\exp(\theta^{k,c}_{i,j})\mathbbm{1}(c=c^*)}{\sum_{c} \exp(\theta^{k,c}_{i,j})} %\mathbbm{1}_{c=c^*}
	\right)
\end{equation}
where $c^*$ is the true source camera model, $\mathbbm{1}(\cdot)$ is the indicator function and $\lambda$ is the relative weight of each scale. In practice, we aggregate across three scales $k=\{3, 4, 5\}$ such that $\lambda_k= \{0.01, 0.0075, 0.005\}$.
After pre-training, we discard the multi-headed classification network and retain only the initialized spatial forensic residual feature extractor trunk. As our ablation study in Sec. 6 shows, this pre-training procedure substantially increases the performance of our network.
