# Supplementary material for: MVFNet: Multipurpose Video Forensics Network using Multiple Forms of Forensic Evidence
Source: arXiv:2503.20991 source file (2025-03-26)
Supplement: Supplementary file 14 [file Supp_FailureModes.tex]

\section{Examples of Failure Modes}
\label{sec:failure_modes}

While our network is robust and can detect many types of video forgeries (splicing, editing, deepfake, inpainting), it can encounter challenges when encountering any of these conditions:
\begin{itemize}
	\item Extreme video compression.
	\item Subtle manipulations that does not noticeable alter the forensic traces, such as remapping the color of one object to another.
	\item Advanced forgery techniques that combines a series of different editing operations, such as those in the VideoSham~\cite{VideoSham} dataset.
\end{itemize}

To further illustrate the difficulties of these conditions, we present examples of them with outputs from our network in Figure~\ref{fig:failure_modes}.
