# Supplementary material for: MVFNet: Multipurpose Video Forensics Network using Multiple Forms of Forensic Evidence
Source: arXiv:2503.20991 source file (2025-03-26)
Supplement: Supplementary file 15 [file Supp_IntermediateResults.tex]

\section{Importance of Different Forensic Modalities}
\label{sec:intermediate_results}

%% Refined by ChatGPT:
Fig.~\ref{fig:intermediate_results} illustrates the discerning power of our network's intermediate layers when facing diverse video manipulations that are all unseen during training. Each type of forgery imparts distinct traces that our network's specialized modules are finely tuned to detect and analyze.

For splicing and editing manipulations (see ``Vid.Sham'' rows), the spatial features, like the spatial forensic residuals, stand out in the intermediate layer results. This is because spliced or edited regions typically maintain temporal consistency across frames, leaving spatial discrepancies as the primary cue for detection. Temporal features, which excel at uncovering temporal inconsistencies, are less pronounced in these cases since the alterations do not significantly affect the temporal flow.

Conversely, inpainting and deepfake manipulations (see ``Inpaint'' and ``Deepfake'' rows) exhibit a higher degree of temporal inconsistency due to the nature of the forgery. In these instances, the temporal features, like the temporal forensic residuals and the optical flow residuals, become increasingly vital, as they can detect the abnormal changes over time that spatial features might miss within a single frame. For deepfakes, however, the network leverages both spatial and temporal features synergistically, capturing the frame-to-frame irregularities in facial features and expressions, providing a robust detection framework.

In addition to showing traces from different forensic modalities, we also included feature maps resulting from our multi-scale hierachical analysis. Here we show the coarsest and finest resulting feature maps in the ``Coarse Features'' and the ``Fine Features'' columns. From these results, we can see that the hierarchical multi-scale approach is able to accurately identify manipulated regions. Furthermore, the prediction from larger scale is refined multiple times, such that the finest scale can accurately localize fake content with very minimal false alarms.
