# Supplementary material for: MVFNet: Multipurpose Video Forensics Network using Multiple Forms of Forensic Evidence
Source: arXiv:2503.20991 source file (2025-03-26)
Supplement: Supplementary file 17 [file Supp_OtherRetraining.tex]

\section{Retraining Competing Forensic Networks}

In our main paper, we compared against 9 state-of-the-art detection systems. These algorithms can be divided into four major groups:
1) Splicing and Editing: MVSS-Net~\cite{MVSS-Net}, MantraNet~\cite{ManTra-Net}, FSG~\cite{FSG},
2) Inpainting: VIDNet~\cite{VIDNet}, DVIL~\cite{DVIL},
3) Deepfake: Self-Blended Images (SBI)~\cite{SBI}, Multi-Attentional Deepfake Detection (MADD)~\cite{MADD}, Cross-Efficient-ViT (CE.ViT)~\cite{CE.ViT}, and
4) General: VideoFACT~\cite{VideoFACT}.
For a fair comparison, we retrained top-performing methods of each group using the exact same training data as ours. We note that we excluded deepfake detectors in this process because they need to isolate and operate on a face, which is impossible in the multi-manipulation setting. Nonetheless, these systems have all seen similar deepfake data as ours.

Therefore, in summary, we retrained MVSS-Net, DVIL, and VideoFACT. In addition, we have to trained VIDNet from scratch due to the fact that model weights for this network were not publicly available.

To retrain MVSS-Net, we used the authors' public code on github to initialize a new model. Next, we trained this model on the video frames in the training portion of our Unified Video Forgery Dataset (denoted in our main paper as UVFA-IND) using the following parameters: \texttt{batch\_size=16, optimizer=SGD, init\_lr=0.0001, decay\_step=2, decay\_rate=0.8}. To obtain these parameters, we performed a grid-search and we chose the set of parameters with the best training loss. Additionally, since MVSS-Net can only accept an input resolution of 512 by 512 pixels, we resized all input frames and ground-truth masks to this resolution before feeding them to the model.

To retrain DVIL, we faithfully reimplemented the authors' public code on github, written in Tensorflow 1.x, in modern Pytorch, and used this reimplementation to initialize a new model. Next, we trained this model on the video frames in the training portion of UVFA-IND using the following parameters: \texttt{batch\_size=4, max\_sequence\_length=4, optimizer=AdamW, init\_lr=0.006, weight\_decay=0.0001, decay\_step=10, decay\_rate=0.5}. To obtain these parameters, we performed a grid-search and we chose the set of parameters with the best training loss. Additionally, since DVIL can only accept an input resolution of 240 by 432 pixels, we resized all input frames and ground-truth masks to this resolution before feeding them to the model.

To retrain VIDNet, we used the authors' public code on github to initialize a new model. Next, we trained this model on the video frames in the training portion of UVFA-IND using the following parameters: \texttt{batch\_size=1, max\_sequence\_length=5, encoder\_optimizer=AdamW, encoder\_init\_lr=0.0001, encoder\_weight\_decay=5.0e-05, encoder\_decay\_step=30, encoder\_decay\_rate=0.1, decoder\_optimizer=AdamW, decoder\_init\_lr=0.001, decoder\_weight\_decay=5.0e-05, decoder\_decay\_step=30, decoder\_decay\_rate=0.1}. These hyperparameters were directly provided by the authors and we found that this set of hyperparameters led to good performance. Additionally, other network hyperparameters are also chosen according to the authors' recommendations in their paper: \texttt{encoder\_base\_model=vgg16\_bn, encoder\_dropout=0.5, encoder\_hidden\_size=512, encoder\_kernel\_size=3, decoder\_dropout=0.5, decoder\_hidden\_size=512, decoder\_kernel\_size=3, decoder\_skip\_mode=concat, max\_sequence\_length=5}. Additionally, since VIDNet can only accept an input resolution of 480 by 854 pixels, we resized all input frames and ground-truth masks to this resolution before feeding them to the model.

And finally, to retrain VideoFACT, we used we used the authors' public code on github to initialize a new model. Next, we trained this model on the video frames in the training portion of UVFA-IND using the authors' originally recommended parameters: \texttt{batch\_size=3, optimizer=SGD, init\_lr=0.001, momentum=0.95, decay\_step=2, decay\_rate=0.5, alpha=0.4}.

We also note that all networks, both pretrained and retrained versions, are subjected to the same benchmarking protocols to ensure fairness in our experiments.
