# Supplementary material for: MVFNet: Multipurpose Video Forensics Network using Multiple Forms of Forensic Evidence
Source: arXiv:2503.20991 source file (2025-03-26)
Supplement: Supplementary file 18 [file Supp_ResultsOnAuthentic.tex]

\section{Qualitative Results on Authentic Media}
\label{sec:results_on_authentic}

In this section, we present our network's ability to correctly classify authentic, unmanipulated video. As shown in Fig.~\ref{fig:results_on_authentic} and many experimental results in our main paper, our network can not only detect manipulated media, but also correctly classify unmanipulated media to be real (authentic). This behavior can be observed as our network will output a higher detection score (close to 1.0) if the input video is forged and a low detection score (close to 0.0) otherwise. Additionally, when our network is given a real video, then its localization result is often an empty, zero matrix, which is a desired outcome.
