# Supplementary material for: MVFNet: Multipurpose Video Forensics Network using Multiple Forms of Forensic Evidence
Source: arXiv:2503.20991 source file (2025-03-26)
Supplement: Supplementary file 19 [file Supp_SpaceTimeComplexity.tex]

\section{Space-Time Complexity Analysis \& Comparisons}
\label{sec:spacetime_complexity}

The table below shows the model sizes \& inference speeds of ours and competing methods. We conducted this experiment using an A100 NVIDIA GPU. We measure the FPS as by dividing the total amount of time to process 1000, 512x512 frames by 1000. From the results shown in Table~\ref{table:spacetime_complexity}, with only 36.5M parameters, MVFNet is among the smallest models. This demonstrates that our superior performance is not due to the size of our network, but rather to the use of novel forensic modalities such as temporal forensic residuals and the innovative multi-scale hierarchical approach in which they are analyzed.
Additionally, while efficiency is not part of our paper's novelties, these results show that
MVFNet's inference speed, measured in frames per second (FPS), is moderate and sufficient for practical applications.

\begin{table}[!t]
	\caption{This table shows the space-time complexity comparisons between ours and other competing methods. With only 36.5M parameters, MVFNet is among the smallest models. This demonstrates that our superior performance is not due to the size of our network, but rather to the use of novel forensic modalities such as temporal forensic residuals and the innovative multi-scale hierarchical approach in which they are analyzed. See more in Sec.~\ref{sec:spacetime_complexity}}
	\label{table:spacetime_complexity}
	\centering
	\resizebox{0.5\linewidth}{!}{
		\begin{tblr}{
				width = \linewidth,
				colspec = {m{16mm}m{18mm}m{7mm}},
				vlines,
				hlines,
			}
			\textbf{ Method } & \textbf{ Params(M) } & \textbf{ FPS }\\
			\textbf{Ours} & \textbf{36.5} & \textbf{11.3}\\
			VideoFACT & 135.4 & 21.6 \\
			MVSS-Net & 146 & 34.3\\
			VIDNet & 337 & 21.8\\
			DVIL & 82.8 & 65.5\\
			MantraNet & 3.8 & 10.1\\
			FSG & 1.2 & 7.1\\
			SBI & 17.6 & 42.4\\
			CE.ViT & 101.4 & 32.1
		\end{tblr}
	}
\end{table}
\begin{comment}
	| Method     | Parameters (M) | FPS  |
	|------------|----------------|------|
	| Ours       | 36.5           | 11.3 |
	| VideoFACT  | 135.4          | 18.6 |
	| MVSS-Net   | 146            | 34.3 |
	| VIDNet     | 337            | 21.8 |
	| DVIL       | 82.8           | 65.5 |
	| MantraNet  | 3.8            | 10.1 |
	| FSG        | 1.2            | 7.1  |
	| SBI        | 17.6           | 42.4 |
	| CE.ViT     | 101.4          | 32.1 |
\end{comment}
