# Supplementary material for: MVFNet: Multipurpose Video Forensics Network using Multiple Forms of Forensic Evidence
Source: arXiv:2503.20991 source file (2025-03-26)
Supplement: Supplementary file 20 [file Supp_StatEvalAblation.tex]

\section{Statistical Evaluation of Ablation Results}
\label{sec:stat_eval_ablation_results}

In this section, we provide additional experimental results showing the statistical variation of the results provided in the ablation study in Table 6 of our main paper.

To achieve this, first, we randomly sample without replacement 5 separate subsets of the \pooleddsabrv-IND's test set used for our ablation study. Then, we benchmarked all variations of our network on each subsets and report the mean and variance of each metrics. We then present our results in Table~\ref{table:stat_eval_ablation_results}.

From the results in Table~\ref{table:stat_eval_ablation_results}, we see that our reported numbers in Table 6 of our main paper remains statistically meaningful. This is because the standard deviations for each metric is small and the mean for each metric is close to what we previously reported.

\begin{table}[!t]
	\caption{Ablation study of the components in our proposed network and their performance evaluations.}
	\label{table:stat_eval_ablation_results}
	\centering
	\resizebox{1.0\linewidth}{!}{
		\begin{tblr}{
				width = \linewidth,
				colspec = {m{40mm}m{17mm}m{17mm}m{17mm}m{17mm}},
				row{2} = {c},
				cell{1}{1} = {r=2}{},
				cell{1}{2} = {c=4}{c},
				cell{3-11}{2-5} = {c},
				vlines,
				hlines,
			}
			\textbf{Setup} & \textbf{\pooleddsabrv-IND} & \\
			& \textit{Reported mAP} & \textit{Mean / Var mAP} & \textit{Reported F1} & \textit{Mean / Var F1} \\

			\textbf{Proposed}   		& \textbf{0.95} & \textbf{0.95 / 0.13} & \textbf{0.77} & \textbf{0.75 / 0.16} \\
			No Spatial Foren. Resid.   	& 0.64 & 0.63 / 0.07 & 0.57 & 0.55 / 0.06 \\
			No RGB Context 		        & 0.82 & 0.80 / 0.10 & 0.52 & 0.55 / 0.07 \\
			No Temporal Residual   		& 0.84 & 0.82 / 0.09 & 0.59 & 0.53 / 0.14 \\
			No Optical Flow Residual    & 0.72 & 0.76 / 0.15 & 0.34 & 0.35 / 0.07 \\
			Standard Transformer 		& 0.86 & 0.83 / 0.06 & 0.56 & 0.55 / 0.02 \\
			No M.S.H Transformer      	& 0.75 & 0.70 / 0.12 & 0.52 & 0.53 / 0.05 \\
			Fine-to-Coarse				& 0.90 & 0.91 / 0.02 & 0.68 & 0.66 / 0.04 %\\
			%            Only Spatial Modalities		& 0.84(-0.09) & 0.21(-0.56) \\
			%            Only Temporal Modalities	& 0.75(-0.18) & 0.42(-0.35)
		\end{tblr}
	}

\end{table}
