# Supplementary material for: MVFNet: Multipurpose Video Forensics Network using Multiple Forms of Forensic Evidence
Source: arXiv:2503.20991 source file (2025-03-26)
Supplement: Supplementary file 21 [file Supp_WholeNetTraining.tex]

\section{Network Training and Hyperparameters}

Our training strategy involves two steps. Initially, we pretrained the Spatial Forensic Residual Module on the camera model identification task with the Video-ACID dataset~\cite{Video-ACID}. Subsequently, we trained the entire network on all types of manipulations present in the \pooleddsabrv-IND dataset.
During training, we started all loss parameters at 1.0 and decayed $\gamma$ by 0.95, $\alpha$ by 0.80, while increased $\beta$ by 1.18 every epoch. Additionally, our optimizer of choice for all training stages is SGD. In the pretraining stage, we initialize the learning rate at $1.00E-03$ with momentum of 0.96 and learning rate decay of 0.65 every 2 epochs. In the full-network training stage, we set the learning rate at $6.00E-04$ with momentum of 0.90 and learning rate decay of 0.85 every 2 epochs. During this final stage, we used the validation detection accuracy as the metric to choose the best checkpoint of our network.
