# Supplementary material for: MVFNet: Multipurpose Video Forensics Network using Multiple Forms of Forensic Evidence
Source: arXiv:2503.20991 source file (2025-03-26)
Supplement: Supplementary file 22 [file Supp_ReviewerRequestedResults.tex]

\section{Additional Experimental Results}
\label{sec:more_exp_results}

In this section, we provide additional experimental results that are specifically requested by our reviewers. Particularly, our reviewers would like to us to evaluate more single-frame based methods that were originally designed for images such as: TruFor, Noiseprint, SpliceBuster, and Adapt-CFA. Since the author of SpliceBuster did not provide official publicly accessible code or model weights, we will only provide benchmarks for the other three methods.

From the results shown in Table~\ref{table:more_exp_results}, we see that our network still obtained state-of-the-art performance on most datasets. It is notable that TruFor slightly outperformed our network on VideoSham. However, this is due to the fact that our network has training examples of splicing and editing. By contrast, TruFor has not only seen more almost twice as many training examples of these type of forgeries, but also TruFor's training examples include more advanced manipulation techniques like Photoshopped image editing and AI-guided splicing.

\begin{table}[!t]
	\caption{Detection and localization performance of methods specifically requested by our reviewers on the \pooleddsname (\pooleddsabrv) and VideoSham~\cite{VideoSham} dataset.}
	\label{table:more_exp_results}
	\pullup
	\resizebox{1.0\linewidth}{!}{
		\begin{tblr}{
				width = 1.0\linewidth,
				colspec = {|m{16mm}|m{27mm}|m{7mm}|m{7mm}|m{7mm}|m{7mm}|m{7mm}|m{7mm}|},
				row{2} = {c},
				cell{1}{1} = {r=2}{},
				cell{1}{2} = {r=2}{},
				cell{1}{3} = {c=2}{0.30\linewidth,c},
				cell{1}{5} = {c=2}{0.32\linewidth,c},
				cell{1}{7} = {c=2}{0.30\linewidth,c},
				cell{-}{3-8} = {c},
				cell{3}{1} = {r=5}{},
				cell{8}{1} = {r=4}{},
				vline{1-3,5,7,9} = {1,2,3-10}{},
				hline{1,2,3,8,10,11,12} = {-}{},
			}
			\textbf{Manip. Group}
			& \textbf{Method} & \textbf{\pooleddsabrv-IND} & & \textbf{\pooleddsabrv-OOD} & & \textbf{VideoSham} & \\
			&  & \textit{mAP} & \textit{F1} & \textit{mAP} & \textit{F1}& \textit{mAP} & \textit{F1} \\
			Splice/Edit
			& TruFor~\cite{TruFor} & 0.74 & 0.47 & 0.79 & 0.57 & \best{0.66} & \best{0.21} \\
			& Noiseprint~\cite{Noiseprint} & 0.49 & 0.08 & 0.32 & 0.12 & 0.50 & 0.09 \\
			& Adapt-CFA~\cite{AdaptCFA} & 0.50 & 0.10 & 0.54 & 0.18 & 0.49 & 0.09 \\
			& MVSS-Net~\cite{MVSS-Net} & 0.66 & 0.29 & 0.45 & 0.14 & 0.56 & 0.10 \\
			& MVSS-Net (R) & 0.94 & 0.77 & 0.63 & 0.09 & 0.52 & 0.01 \\
			General
			& VideoFACT~\cite{VideoFACT} & 0.78 & 0.36 & 0.74 & 0.28 & 0.54 & 0.07 \\
			& VideoFACT (R) & 0.88 & 0.50 & 0.79 & 0.39 & 0.55 & 0.08 \\
			& Ensemble of (R)* & 0.90 & 0.54 & 0.73 & 0.44 & 0.52 & 0.11 \\
			& \textbf{Ours} & \best{0.95} & \best{0.77} & \best{0.91} & \best{0.59} & 0.63 & 0.14
		\end{tblr}
	}
\end{table}
